# Supplementary material for: Spatiotemporal distribution of the glycoprotein pherophorin II reveals stochastic geometry of the growing ECM of $Volvox~carteri$
Source: arXiv:2412.05059 source file (2024-12-06)
Supplement: Supplementary file 1 [file PhII_SI_Ray.pdf]

# SI Appendix: Spatiotemporal distribution of the glycoprotein pherophorin II reveals stochastic geometry of the growing ECM of *Volvox carteri*

Benjamin von der Heyde,[1,*] Anand Srinivasan,[2,*] Sumit Kumar Birwa,[2] Eva Laura von der Heyde,[1] Steph S.M.H. Höhn,[2,†] Raymond E. Goldstein,[2,‡] and Armin Hallmann[1,§]

[1] *Department of Cellular and Developmental Biology of Plants, University of Bielefeld, Universitätsstr. 25, 33615 Bielefeld, Germany*
[2] *Department of Applied Mathematics and Theoretical Physics, Centre for Mathematical Sciences, University of Cambridge, Wilberforce Road, Cambridge CB3 0WA, United Kingdom*

(Dated: December 6, 2024)

This file includes supporting text, Figs. S1 to S11, Tables S1 to S2 and SI References.

* Joint first author
† sh753@cam.ac.uk
‡ R.E.Goldstein@damtp.cam.ac.uk
§ armin.hallmann@uni-bielefeld.de

## 1. SUPPLEMENTARY DATA: PHEROPHORIN II OVERVIEW AND DNA SEQUENCES

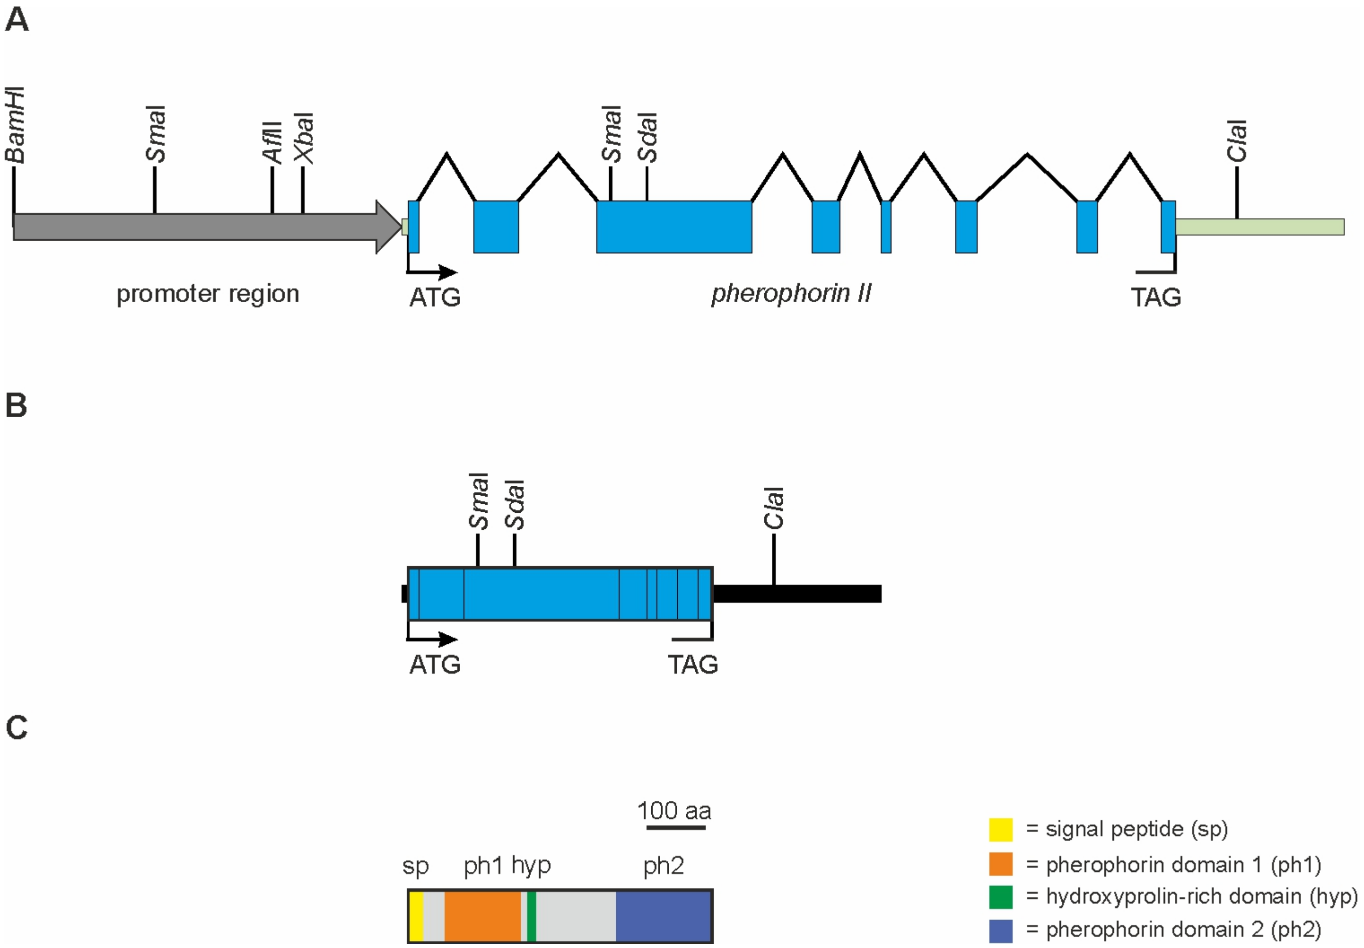


FIG. S1. **Schematic structure of the *phII* gene, *phII* mRNA and pherophorin-II protein.** (A) The genomic region schematized here corresponds to the 8329-bp genomic fragment utilized in plasmid pPhII-YFP. The *phII* gene [S1] is located on scaffold 34 (nucleotides 980223 to 985045) of the *V. carteri* genome version 2.1 [S2] in Phytozome v13 [S3] on the reverse strand. The start codon is at nucleotide position 985025-985027 on the reverse strand. In the current *Volvox carteri* genome annotation available at Phytozome v13 (Volvox v2.1) pherophorin II is not annotated. Therefore the gene structure was established based on older annotations and confirmed with RNA-Sequencing data [S4]. The gene structure is indicated as follows: Coding sequences are represented by blue squares, intron sequences by carats, UTRs by green bars and the promoter region by a grey arrow. Start (ATG) and stop (TAG) codons are highlighted. The given restriction sites are also marked in SI Appendix, Fig. S2, which represents the genomic sequence of the *phII* gene. (B) Structure of the *V. carteri phII* mRNA. Sequence features are as indicated in A. The coding sequence (blue squares) totals 1557 nucleotides. The 5' UTR is 18 bp in length, while there is a quite long 3' UTR of 869 bp. The complete mRNA is 2,444 nucleotides in length. (C) Structure of the *V. carteri* pherophorin-II protein. The polypeptide comprises 518 amino acids and the calculated molecular weight amounts to 54.5 kDa. As pherophorin-II is an extracellular protein, it possesses a cleaved N-terminal signal peptide (sp) of 24 amino acids. In the mature protein three domains can be identified: an N-terminal pherophorin domain (ph1) with an E-value of 4.5e-27, a hydroxyproline-rich domain (hyp) in the middle [S5] and a C-terminal pherophorin domain (ph2) with an E-value of 2.1e-32.The pherophorin domains where identified by blasting the Pfam database [S6] using the hmmscan function [S7]. The short Hydroxyproline-rich domain consists of 78% (hydroxy) prolines (seven of nine amino acids).

**GGATCC**ATGACTGGAAAACCCATCCATGACCAAGTCGTTCCCCGAGAGATAGCAGCTTTGGATCGACT ***BamH*I**

CGTCGCTTGTGAAAGCCTACCTGGTTACTTAGACGGATTTAGCGACTAGACCACTTATGAAGGTGTTG

ATAAACACCGGGGGTTTCCCTTGGGGTTTTATAGTCGCTTGCAGTCCGTCTGAGGCGCTCGGGATAAT

ATGCCGTACAGTAGTAGATATTCCTGCAGAAGAGAGTCGCACCTCCAGGGAAGAGTTACAATACAGGT

CTGGCCGTGAACGGGCAGACGTGTACAAGATGGTGTACGGAATCGAGTATGTGCACGGATCGTTACAG

CCATGGCCGTAGCCATGTACTGCTGAGTACGGCTGTAGTCGAAAGATGACGAAGATAAGATAGTTTTA

TGTACTGTGTGTACGATATTCGCCTCGACGATGGAATGATAAGAAGGAATGGAGTCCCTACTCGGAAG

TCCTGAGCCAGGCTCTTACACTGGGCACACATTGCCATCCAATGGATGGCCATGTGAATCACAGTGGT

GCCCGGCCTAAGGTAGCTAAGGACTTGGCCGTTATCATCGGTAGATTGCTCACCCACCTTCTCCGACC

AGGAAAACATCCTCGTCACTGGTGCACAGCTCGTCATAGCGATGAATGTTGCAGGGGTGCAAAGGCAA

GTTCCACCACACCATTATGAGCAACCTTAGGACCGCGTTCC**CCCGGG**TAGACACAGGAGGTTTCAGGG ***Sma*I**

GCTAGATATACTGGTCCAATAAGCAGGGTGCTATTGATGTAGGCAGTAATGTAGCACCCTCCCTCATC

CGACGTACCTCACTCCCTGCACATGTAGAGCCCCTGCGTAGAACGGCTATCTGTGATGAGGGGGAGTC

CCTGGTATAGAGGCCAATGGGAGCATGTGCCGTTGTTGGGCATTCGAGGGGTGCGTGACAGCGTTGTC

ATCGGTAGGGTCGTGCCGAGTTGTGAAGACGGGCTCCTGTAATGGGCCTTATCATGCAGTAGGTTTCT

TGTGGTTTCCGAGGCCGAGGTCATTTTGCCGGGGTGTACGGCATTGTTGCGGGTTGCGGGAAGTTGTA

CAGGTAAATGCATCGGCCATTTTTATCAGCCTTGTTTAAATATAAGTAGACAACCGAGCAAGAACCAA

AGTTTGTCGGAAAGAATTTGGGCAGAGGCCGAAGCTCGCCTGGCAAGCACTGCGCTGAAGGGATAGAG

AGAGACACGAATAAGAAGTGTACAACGGGGCCTCAATAGGCTTTGGGGTCCAGATCGCTGACGCCCTC

GCTCTCAGGCATCAAGTCCCGGACATGGGC**CTTAAG**ACCTGGAGTTGCTGGGCTATTCCCTCTCGCCC ***Afl*II**

TCCCCGCTCTGACCACTATCCCTCTCTCCAGTTCCCTTTCAGTTCGGGTGGTGCAACGCCAGGCCCCT

CGCCACACACACCGCACCGCACCCACGTTTGTTAAGCGCTAGCAGGCTGTTG**TCTAGA**GCTGTAGAAG ***Xba*I**

TTCCTAGGTCTATGTTGATGTAGTTTGGTCCCGTTGCTGATGCAACTGGCTTTCGCATCATTAACCGC

CGAGTAGCAGCCGTAGCTACCGGTGCGGAAAGGATGCATGCTCACCAACCGAAATGATGAAGTGCGTG

TGGCGAAGTTATATTCATTATGCCAGGATCAGAGATGTTGGTCAGTAAATAGCAAGTTATATAAAAGG

AATGGTGCTACAGATTACAACGACGGGTCGGATTCCGAAACGTACAACACGAGCAACATCCCAACGGA

TGAAATGCACATTTATATGTGTCCGCGACTAAC**GAATTC**TGCGCTGTGTTTCTAAGATTTATATTCTG ***Eco*RI**

CATAAAGATATTGATTCCAAAGGACGAAGCGCCTCTGTTGCGGTGGCCAGTCTCGGAAGCGGCTACCT

GCGCCCGCCGTTTACGGTAGTCGTACGGCCCCGCAGCAGCACAGCTGCCGCGGTCGGTCGGGTAGATA

AATAGCGCCACTATGATACAGAACATCATCAAAGTGACATAGCTCTGACAAT**ATG**GCATACTTTGCAA **start**

AGGTAGCTTTCATTTTGGCGACAGCGCTGGCGGTTGGCTGGTGCGTTTTTAGCATGGTGCATTCCCAT

ATGCCTGGGCTTACAATCTGAGGTTGGGTCTATATATTTAAGTATATTTAAGAGCCATATACTTGAAG

GCTTTCAGTCTTTGCCTTTGCGTCGCAAAAGACGTACATGTCCTGTCGCATGCCATAGTGATGAGCCT

TTTCTATAAAGCAATACATAAAAGATAAGACGTCTACAATCATAACTCGATCATGAAACAGCAAGCGT

CAACCATGAGCACTGACCTTGCTTGCTGCTTGTCGCCGCTGGTTCCAGGGCGCTCAGCGCTCATGCGC

AGGAATACAACGAGTACGATCCCTCAGCTGTCACGCCTGGCAGCATCCCCAACTTCCCATTCCGCGAC

TGCAACACCACAAACGGCGCGTACCGGCTGGCACCGGTGTGGCGGCCTTCGGGCAGCAACACGTACTG

CTTCAAGATCCAGGTCAGCCAGGATGCCCTGTCCTGCACTGGCGCCTGCTGCAGCGCCGACTTGCACA

AAATTGAGGTGAGCCCACGGCCGGCTGATGGTGTGGGGGATGCGACATGCGGACACAGTGCTACAGGT

CCTAGGGCCTCGGAAAGCACGGGAAGAGGCTCATTGGGCCCGCAACCAAATGTCAACGATTATTTTCC

AGTAGTTTCTCATGTGTGTGTGTGTGTGCATGTGCGCATGATGTCGGTGTTGAGGGCTCCGTTACCAT

CCTAGCTGCTCCTCCGGGGAAGTGGATTTCTAATCAGGGTTCGGAACGCGCCTCACAATATTTACATA

GCTCATTTACATGTGCTGGAGAGAATGAGAAGTTCGCACCCTCAAAAGTAGAGGGAACATCAAATTGT

GATGTTCCCTCCTGCCTCACCTTGCCCTTACTCCATCCTCCCACCACATGCCACCCCGCCATGTCCGC

AGTTCAACGTGTCCAGCAGCTGCCTGGTGGCCGGGGCCTCAGTTGTCGCCACCGTGAATGGAGTGCGG

A**CCCGGG**TTGGTGCGACCCTGGACAAGGCCCCGGCTGGGCCTGTTGGCTCCGCCGTTCTGCGGCTCAC ***Sma*I**

CCAGCTGGGGCTGGACACCACGACCGCCCAGGATGCGGAGGTGTGCCTCACCCTCAAGACCAACCGCG

GAGGCCAGGGCTGCACCACCCTGGAGCAACTGTGCTCGTCGCCAGGCTTCCCTGCAGGGACATGCACA

GCAGCTATGTTCGATGTCGCGTGTGATTGCTGCCCGGTTTCTCAAGCCGGTCAGGCCCTCCCGCCGCC

GCCACCAGTTATTCCGCCGGTCTTCCGGCCTTGTGACGTCTGCATCGCCGCGACCATTGTGCCCCCGG

CCAATGATGTGCGACCATACCGCTACGACAGCGCCACCTGCGCCGCCATTCAGCAGAACATCGCCGAT

GCCATGAACTCTCTCCTGGGAGGCGCCAACATCGGCGCCTTCTCACCTTTCGCGCCAAATGCAAGCCA
GTGCTTTGACACACAAATCATTACATGTGGCAGGTTCAACGGTTCGGACAGTGATGCGTTGGCCAATC
TGACGGAAGCAGTGCAGCAGCAGCTTTCCGCCTTCATTGGAGTCGCGTCTGGCGGCAACGTCTGCAAT
CCAAAGTTGGAGAAATACACGGTGACGGTCTCCACCATCAACAATGTAGCAGATCAGTGCCTGGACCT
CTCGCAGTCGGCTAGTTGCTTCCTGCCTGGCGTTCCATTCCCCAACTGCACGTGAGTCACCCTACTTC
ATGGCGTCGTCTCTTTTGCGGCGCGGCCGCCCTCCGTAAAGATTTGGGGGCGAGGATGTAGGGCCTAA
TAACCAAAGCTTCCCCCCGCAATGGATGGACCCATGTTTGGGATCTGGCTAGCGTCTTTGTCGTGTAT
GCAGAGCTTTGGATGAATGGCTGAAGGCAAAGACACCGCGCTTGCATGGATACCTTGCTCACATGGCT
ATTTGAAAAAATCAGGAACGTTGGGTGAATATGTGATAGTACTAGTTACCGACCCTGCTGCCGCCTCC
GCTCGCCCTCTGACGCGCAGGTGCAACACAACCCAGGGAGTCATGCCGTTCACAGTCTCCCCCACCTG
GTATGCACAGCCGGCCAATGTGCGCTGGGGCCGCAACGTCACTGAGTACTGCTTCACCGTCAACACGC
TACAGCCAAGTCAGGTCGTGCCGGTGAGGCCAGATAGGTGCATGGAGGACCCGTGGGGTGGCGCTTTG
TTTTCTTCCACGCACCCATGCATGCTTGGCTGCATGCCTGATGAGCTCGGTTAGTTGTATCGGGTCTG
GACAAGGCACACGGGCCTGTCTGCTGCGCGTAGCTCACCCAGACAAAGTTAAGAAATTACATGACTGA
GGATGCTGCCTCGTTCGCTGTCCCCCTGCAGAGCACCTGCTACAACGCAAACGACGCGCTCGCCAAGA
TCGAGTGGTATGCAAGTAAGTTATCATTGCTGTTGCTTGCTTGCGTAGTCTTCTATCGTTTCAACGTT
TCTTAGATAAGACCCGTCCTTTCAACCTGGGCAGACATGCATGGATATGTGGGAGTACGGCATGCGAA
TGGATATGGATATGTGCAAACTTCTACTGTCGCAGCATGATGTGAACTCTGGCCCTGCCGGCTGCACA
CATACGCATACATGACTTCCGTAATGCGAGCAGACTGCAGCATAGCACCCAGTACGGCAGCATCAGTG
GTTAACCTTTTTTGGTCCTCGCTACAGCCTAGGGTTTCACCTGCCGTGCATTTTGGCTTGTGTTTCCA
TGACTGCAGGTGATGCGTTCAGGTCGGCGGTCAAGGGTTTCACGGTGTACCCCGCCGGGGGATCAAAC
AAGACCATTGCCGACAGCTGGGGCGCCACTGGAACCGATACCCTGAAAGGTGAGGCCGGCAAGCTAGA
TAGCAGCTCAGGTAGATGCACCTCGTGCGGGGCTCATTCGCTGCTTCGATTGTGGATTCTGTGCGGCA
CTTACCTGCCGTGTGTCACAAGGGTAACTGTCGTGCGAGACCTTCACTTACAATACACTCGAGGAAAT
CTCGACGGACCTGCATCTCGGAAGGCCTCTTCGATGACCCTATCAAAAGATCAGCAATAAGCTCCAAC
AGTGTATGAAGATTGACGGAGCTGTCAAGCTCAATAACATAATCCCGAAAATGGCAAGCACTACGGCT
ACTGTATAAAACCCAGCGCAGAGGCTACACTCCCTTCGCTCCTGGCGCATCTAAGCTGCAATTACAAT
TACAGTAACTCTGTTCAGTAGCCAGCCATGCGCCGGTTTGTTTGTACCGTACCTGTCCAATTGCCATG
TGCTGCACCATCACTGCTAATGCCTGCATGTCAAATAAGATCACATCGTTCCCTGCCTGCGCATCCTT
TTGTTCGTGTGTGCAGTCAATCTCAACTGGAACCTGCTGCAAGCCAACGGCGGCAAGGTTTGCGTGGC
GATTCAGAACCCGTTCACCATGGGCGACATCTGCAAGGGAGCCCTTGGCCAGTGGTAAGTCCTGAGGC
AGGGGTTTGCGAGGCCTATCCTTCTCAACTCAACTAAGATGACCTCCCGCGTACCCGCATCAATACCA
ATACAACGTCCATGGCCCCCCCGGCTTTTACGGACACACCTGCACTTGTGTGCGGAACTTGTAACTTG
TAACTAACGAATGTACGGCCGCGCCACGTGCAAGAA**ACGCGT**TTTCCTTCCCGCACTTTTAGACCACA ***Mlu*I***
AGTTGCACACGTGTCAATTAGCAGCAGTGGTAGTAGGGATGAGTGTGCCTGATTGCTATGTCGCTAAT
AATACTCCTTCATGCCCCTGCTGTATCTTGCCTGCGCCCGTGCAGCTACGCCAGCATCTTCAACAGGG
ACAACTCGGACTACTGCTGCCCCATCTACCGCACGGGGCCA**TGA**TTGCCGTAAGAGCAGTCATGGCGC **stopp**
TGGAGAGCGCAGCAGCCGGAAGTAGGGGTAGAAGTTGTTGTTGCTACAAGTGCAGCAGCAGGCAGAAG
ATAAGGAGCACAATATGGCATCTTAGTACTGCATGAATGAACTGACATACAGACATGTTTACAGATCA
TCAGTCGGCGGGTTTTTCACTTTATCTCTTCGTTCGGTTGCAGCAGTCGATAGATAGATAGACAGACG
AGCTAGACAGTATGATTGATCTGTTGGACGGAATCTTTTCCTTTCCCCGACACAACTGCTTGTAGTAA
CATTTTTTGTAATGATTT**ATCGAT**GTACCACAATTCCTCTCGAACAGTTACGAGGCTAGATACTCGGA ***Cla*I***
CAGGCCTGGTAGGCAGGTGCTGCTGTGCTGCATATATCTATTAGGATGGTGGCGCAGAGGTTTCTTTG
GTGGGTTTGCATGTTGCCATAGACACCGCGGCCGGATGTGCACGGTTTATTAAATGATAATGTGGCTT
GTGAAATTAACGCAAGTAGCTGGCGAGCAGTGGCTACTTGGTCAAGTGGACTGAGTCTGAGCATGACG
TGGTGGGACGCGGTGCGGTCTATTTGGAGCACTAAAGTACATCTCGTCATCAGCAGGCTCTGCTGGGT
CCTGCGGGTGGCGCAAGTTTGAAACGAACGCGCGGTGGCACATTCTCGTGGGTGTCTTCACCAAGGAG
TTCCAAATCCTAAGAACAAGGTTAGCCCAATGGAACTGCAGTGGCGTCTGAGGTAGCTGACGGTAGAG
ACAGATCACGGTGATACAGTAACCTTTTACCGGGGCACATTGTGGCGACTGGAGCCGCATGACCGTCC
CCGTCACTTTGTAACCGCTCAAACTGCACGATAACTCCAACCCACACCGTCTTCAATGCGGCAGCTTG
CGACGGTTTCGC**AGATCT**TCCGAACTGCTCCAATAGCAGCTTGGGATCGACCCGTCATTTCTGCACCA ***Bgl*II**
AGTCGCAAAATAATGACAGATCCTAGGTGGCCGTGGTTATATGCTTTGCCACGTTGTAGAGTCCGAAC
TATATTGTCTTCCCTATGGGCACCCATGGCCATGCTGGATGGCGAAGCACAGTGGTGAGCGGCCTAAG

GTAGCTCTCCGACCAGGAAAACATCACCAGTGCACAGCTCGTCATAGCGATGAATGTTGCAGGGGTGC
AAAGGCATGTTCCACCACACCATTACGAGCAACCTTAGGACCGCGTTCCCCCAGGTAAACAGGGGAGG
TTTCAGGGGCTAGATATACTGGTCCAATAAGCAGGGTGCTATTGATGCAGGCGGTAATGTAGCACCCT
CCCTCATCCGACGTACCTCACTCCCTGCACATGTAGAGCCCCTGCGTAGAACGGCTATCTGTGATGAG
GGGGAGTCCCTGGTATAGAGGCCAATCATGCAAACTCGCTGTGCAGTGCTTCATCAGTTAGGGAGCAT
GTGCCGTTGTTGGACATTCGGGGACTGCGGGACAGCATTGTCAACATCGTTGCAGGCCCTGTAATGGG
CCACATCATGCAGTAGGTTTCTAGCGGTTTCCGAGGCCGAGGTCATTTTGCCGGGGTGTACGGCATTG
TTGCGGGTTGCGGGAAGTTGTACAGGTAAATGCACCGGCCACATTTACCAACATTGCTTTAAATATAA
GTAGACAACCGAGAAAGAACCAAAAGATGTCGGAAAGAATTTGGGCAGAGGCCGAAGCTCGCCTGGCA
AGCACTGCGCTGAACGGATAGAGAGAGACACGAATAAGAAGTGTACAACGGGGCCTCAATAGGCTTTG
GGGTCCATAGATACCGGGCGCCCTCGCTCTCAGGCATTAAGTCTCGGACGCGGGCCACAAGACCTGGA
GCTGCTTGGCTGTTCCCTCTCGTCCCCCCCCTTCAGAAGAAAAACTCTGACCACTATCCCTCTCTCCA
GTTCCCTCTCAGTCTGGGTGGTGCAATACCAGACCCCTCGCCACACACACCGCCACCTCAGCACCAAA
CCGTCACATTACGCTGCAAACATTGAGTCACGTTTGTTAGGCGCTAGCACGCTGTTGTATGAATTAGT
TTCTGAGTCTATGTTGATGTGGTTTGGTCCCGTTGCTGATGCAACTGGCTTTCGCATCATTAACCGCC
GAGTAGCAGCCGTAGCTACCGGTGCGGAAAACGATGCATGCTCACCAACCTAAATGATGAAGGGTGTG
TGGCGAAGTTATATTCATTATGCCAGGATCAGAGCTGTTGGTCAGTAAATATCAAGTTATATAAAAGA
AATGGTGCTACAGATTACAACGACGGGTCGGATTCCGACACGTACAACACGAGCAACATCCCAACGGA
TGAAATGCACATTTATATGTGTCTGCGATTAAC**GAATTC** ***Eco*RI**

FIG. S2. **Genomic sequence of the *V. carteri phII* gene.** The sequence depicted here corresponds to the 8329-bp genomic fragment utilized in plasmid pPhII-YFP. The *phII* gene [S1] is located on scaffold 34 (nucleotides 980223 to 985045) of the *V. carteri* genome version 2.1 [S2] in Phytozome v13 [S3] on the reverse strand. The start codon is at nucleotide position 985025-985027 on the reverse strand. In the current *Volvox carteri* genome annotation available at Phytozome v13 (Volvox v2.1) pherophorin II is not annotated. Therefore, the gene structure was established based on older annotations and confirmed with RNA-Sequencing data [S4]. The gene structure is indicated as follows: Coding sequences are shown with blue background, UTRs with green background and the promoter region with grey background. Start and stop codons are highlighted (violet font). The 5' UTR is just 18 bp in length, while there is a quite long 3' UTR of 869 bp. The coding sequence totals 1557 nucleotides. The restriction sites that are shown in Figure 2 (main text) and SI Appendix, Fig. S1 A and B are marked (bold, underlined). Restriction sides that were used for inserting the *yfp* coding sequence are marked with asterisks.

**GGATCC**ATGACTGGAAAACCCATCCATGACCAAGTCGTTCCCCGAGAGATAGCAGCTTTGGATCGACT *BamH*I
CGTCGCTTGTGAAAGCCTACCTGGTTACTTAGACGGATTTAGCGACTAGACCACTTATGAAGGTGTTG
ATAAACACCGGGGGTTTCCCTTGGGGTTTTATAGTCGCTTGCAGTCCGTCTGAGGCGCTCGGGATAAT
ATGCCGTACAGTAGTAGATATTCCTGCAGAAGAGAGTCGCACCTCCAGGGAAGAGTTACAATACAGGT
CTGGCCGTGAACGGGCAGACGTGTACAAGATGGTGTACGGAATCGAGTATGTGCACGGATCGTTACAG
CCATGGCCGTAGCCATGTACTGCTGAGTACGGCTGTAGTCGAAAGATGACGAAGATAAGATAGTTTTA
TGTACTGTGTGTACGATATTCGCCTCGACGATGGAATGATAAGAAGGAATGGAGTCCCTACTCGGAAG
TCCTGAGCCAGGCTCTTACACTGGGCACACATTGCCATCCAATGGATGGCCATGTGAATCACAGTGGT
GCCCGGCCTAAGGTAGCTAAGGACTTGGCCGTTATCATCGGTAGATTGCTCACCCACCTTCTCCGACC
AGGAAAACATCCTCGTCACTGGTGCACAGCTCGTCATAGCGATGAATGTTGCAGGGGTGCAAAGGCAA
GTTCCACCACACCATTATGAGCAACCTTAGGACCGCGTTCC**CCCGGG**TAGACACAGGAGGTTTCAGGG *Sma*I
GCTAGATATACTGGTCCAATAAGCAGGGTGCTATTGATGTAGGCAGTAATGTAGCACCCTCCCTCATC
CGACGTACCTCACTCCCTGCACATGTAGAGCCCCTGCGTAGAACGGCTATCTGTGATGAGGGGGAGTC
CCTGGTATAGAGGCCAATGGGAGCATGTGCCGTTGTTGGGCATTCGAGGGGTGCGTGACAGCGTTGTC
ATCGGTAGGGTCGTGCCGAGTTGTGAAGACGGGCTCCTGTAATGGGCCTTATCATGCAGTAGGTTTCT
TGTGGTTTCCGAGGCCGAGGTCATTTTGCCGGGGTGTACGGCATTGTTGCGGGTTGCGGGAAGTTGTA
CAGGTAAATGCATCGGCCATTTTTATCAGCCTTGTTTAAATATAAGTAGACAACCGAGCAAGAACCAA
AGTTTGTCGGAAAGAATTTGGGCAGAGGCCGAAGCTCGCCTGGCAAGCACTGCGCTGAAGGGATAGAG
AGAGACACGAATAAGAAGTGTACAACGGGGCCTCAATAGGCTTTGGGGTCCAGATCGCTGACGCCCTC
GCTCTCAGGCATCAAGTCCCGGACATGGGC**CTTAAG**ACCTGGAGTTGCTGGGCTATTCCCTCTCGCCC *Afl*II
TCCCCGCTCTGACCACTATCCCTCTCTCCAGTTCCCTTTCAGTTCGGGTGGTGCAACGCCAGGCCCCT
CGCCACACACACCGCACCGCACCCACGTTTGTTAAGCGCTAGCAGGCTGTTG**TCTAGA**GCTGTAGAAG *Xba*I
TTCCTAGGTCTATGTTGATGTAGTTTGGTCCCGTTGCTGATGCAACTGGCTTTCGCATCATTAACCGC
CGAGTAGCAGCCGTAGCTACCGGTGCGGAAAGGATGCATGCTCACCAACCGAAATGATGAAGTGCGTG
TGGCGAAGTTATATTCATTATGCCAGGATCAGAGATGTTGGTCAGTAAATAGCAAGTTATATAAAAGG
AATGGTGCTACAGATTACAACGACGGGTCGGATTCCGAAACGTACAACACGAGCAACATCCCAACGGA
TGAAATGCACATTTATATGTGTCCGCGACTAAC**GAATTC**TGCGCTGTGTTTCTAAGATTTATATTCTG *Eco*RI
CATAAAGATATTGATTCCAAAGGACGAAGCGCCTCTGTTGCGGTGGCCAGTCTCGGAAGCGGCTACCT
GCGCCCGCCGTTTACGGTAGTCGTACGGCCCCGCAGCAGCACAGCTGCCGCGGTCGGTCGGGTAGATA
AATAGCGCCACTATGATACAGAACATCATCAAAGTGACATAGCTCTGACAAT**ATG**GCATACTTTGCAA **start**
AGGTAGCTTTCATTTTGGCGACAGCGCTGGCGGTTGGCTGGTGCGTTTTTAGCATGGTGCATTCCCAT
ATGCCTGGGCTTACAATCTGAGGTTGGGTCTATATATTTAAGTATATTTAAGAGCCATATACTTGAAG
GCTTTCAGTCTTTGCCTTTGCGTCGCAAAAGACGTACATGTCCTGTCGCATGCCATAGTGATGAGCCT
TTTCTATAAAGCAATACATAAAAGATAAGACGTCTACAATCATAACTCGATCATGAAACAGCAAGCGT
CAACCATGAGCACTGACCTTGCTTGCTGCTTGTCGCCGCTGGTTCCAGGGCGCTCAGCGCTCATGCGC
AGGAATACAACGAGTACGATCCCTCAGCTGTCACGCCTGGCAGCATCCCCAACTTCCCATTCCGCGAC
TGCAACACCACAAACGGCGCGTACCGGCTGGCACCGGTGTGGCGGCCTTCGGGCAGCAACACGTACTG
CTTCAAGATCCAGGTCAGCCAGGATGCCCTGTCCTGCACTGGCGCCTGCTGCAGCGCCGACTTGCACA
AAATTGAGGTGAGCCCACGGCCGGCTGATGGTGTGGGGGATGCGACATGCGGACACAGTGCTACAGGT
CCTAGGGCCTCGGAAAGCACGGGAAGAGGCTCATTGGGCCCGCAACCAAATGTCAACGATTATTTTCC
AGTAGTTTCTCATGTGTGTGTGTGTGTGCATGTGCGCATGATGTCGGTGTTGAGGGCTCCGTTACCAT
CCTAGCTGCTCCTCCGGGGAAGTGGATTTCTAATCAGGGTTCGGAACGCGCCTCACAATATTTACATA
GCTCATTTACATGTGCTGGAGAGAATGAGAAGTTCGCACCCTCAAAAGTAGAGGGAACATCAAATTGT
GATGTTCCCTCCTGCCTCACCTTGCCCTTACTCCATCCTCCCACCACATGCCACCCCGCCATGTCCGC
AGTTCAACGTGTCCAGCAGCTGCCTGGTGGCCGGGGCCTCAGTTGTCGCCACCGTGAATGGAGTGCGG
A**CCCGGG**TTGGTGCGACCCTGGACAAGGCCCCGGCTGGGCCTGTTGGCTCCGCCGTTCTGCGGCTCAC *Sma*I
CCAGCTGGGGCTGGACACCACGACCGCCCAGGATGCGGAGGTGTGCCTCACCCTCAAGACCAACCGCG
GAGGCCAGGGCTGCACCACCCTGGAGCAACTGTGCTCGTCGCCAGGCTTCCCTGCAGGGACATGCACA
GCAGCTATGTTCGATGTCGCGTGTGATTGCTGCCCGGTTTCTCAAGCCGGTCAGGCCCTCCCGCCGCC
GCCACCAGTTATTCCGCCGGTCTTCCGGCCTTGTGACGTCTGCATCGCCGCGACCATTGTGCCCCCGG
CCAATGATGTGCGACCATACCGCTACGACAGCGCCACCTGCGCCGCCATTCAGCAGAACATCGCCGAT

GCCATGAACTCTCTCCTGGGAGGCGCCAACATCGGCGCCTTCTCACCTTTCGCGCCAAATGCAAGCCA
GTGCTTTGACACACAAATCATTACATGTGGCAGGTTCAACGGTTCGGACAGTGATGCGTTGGCCAATC
TGACGGAAGCAGTGCAGCAGCAGCTTTCCGCCTTCATTGGAGTCGCGTCTGGCGGCAACGTCTGCAAT
CCAAAGTTGGAGAAATACACGGTGACGGTCTCCACCATCAACAATGTAGCAGATCAGTGCCTGGACCT
CTCGCAGTCGGCTAGTTGCTTCCTGCCTGGCGTTCCATTCCCCAACTGCACGTGAGTCACCCTACTTC
ATGGCGTCGTCTCTTTTGCGGCGCGGCCGCCCTCCGTAAAGATTTGGGGGCGAGGATGTAGGGCCTAA
TAACCAAAGCTTCCCCCCGCAATGGATGGACCCATGTTTGGGATCTGGCTAGCGTCTTTGTCGTGTAT
GCAGAGCTTTGGATGAATGGCTGAAGGCAAAGACACCGCGCTTGCATGGATACCTTGCTCACATGGCT
ATTTGAAAAAATCAGGAACGTTGGGTGAATATGTGATAGTACTAGTTACCGACCCTGCTGCCGCCTCC
GCTCGCCCTCTGACGCGCAGGTGCAACACAACCCAGGGAGTCATGCCGTTCACAGTCTCCCCCACCTG
GTATGCACAGCCGGCCAATGTGCGCTGGGGCCGCAACGTCACTGAGTACTGCTTCACCGTCAACACGC
TACAGCCAAGTCAGGTCGTGCCGGTGAGGCCAGATAGGTGCATGGAGGACCCGTGGGGTGGCGCTTTG
TTTTCTTCCACGCACCCATGCATGCTTGGCTGCATGCCTGATGAGCTCGGTTAGTTGTATCGGGTCTG
GACAAGGCACACGGGCCTGTCTGCTGCGCGTAGCTCACCCAGACAAAGTTAAGAAATTACATGACTGA
GGATGCTGCCTCGTTCGCTGTCCCCCTGCAGAGCACCTGCTACAACGCAAACGACGCGCTCGCCAAGA
TCGAGTGGTATGCAAGTAAGTTATCATTGCTGTTGCTTGCTTGCGTAGTCTTCTATCGTTTCAACGTT
TCTTAGATAAGACCCGTCCTTTCAACCTGGGCAGACATGCATGGATATGTGGGAGTACGGCATGCGAA
TGGATATGGATATGTGCAAACTTCTACTGTCGCAGCATGATGTGAACTCTGGCCCTGCCGGCTGCACA
CATACGCATACATGACTTCCGTAATGCGAGCAGACTGCAGCATAGCACCCAGTACGGCAGCATCAGTG
GTTAACCTTTTTTGGTCCTCGCTACAGCCTAGGGTTTCACCTGCCGTGCATTTTGGCTTGTGTTTCCA
TGACTGCAGGTGATGCGTTCAGGTCGGCGGTCAAGGGTTTCACGGTGTACCCCGCCGGGGGATCAAAC
AAGACCATTGCCGACAGCTGGGGCGCCACTGGAACCGATACCCTGAAAGGTGAGGCCGGCAAGCTAGA
TAGCAGCTCAGGTAGATGCACCTCGTGCGGGGCTCATTCGCTGCTTCGATTGTGGATTCTGTGCGGCA
CTTACCTGCCGTGTGTCACAAGGGTAACTGTCGTGCGAGACCTTCACTTACAATACACTCGAGGAAAT
CTCGACGGACCTGCATCTCGGAAGGCCTCTTCGATGACCCTATCAAAAGATCAGCAATAAGCTCCAAC
AGTGTATGAAGATTGACGGAGCTGTCAAGCTCAATAACATAATCCCGAAAATGGCAAGCACTACGGCT
ACTGTATAAAACCCAGCGCAGAGGCTACACTCCCTTCGCTCCTGGCGCATCTAAGCTGCAATTACAAT
TACAGTAACTCTGTTCAGTAGCCAGCCATGCGCCGGTTTGTTTGTACCGTACCTGTCCAATTGCCATG
TGCTGCACCATCACTGCTAATGCCTGCATGTCAAATAAGATCACATCGTTCCCTGCCTGCGCATCCTT
TTGTTCGTGTGTGCAGTCAATCTCAACTGGAACCTGCTGCAAGCCAACGGCGGCAAGGTTTGCGTGGC
GATTCAGAACCCGTTCACCATGGGCGACATCTGCAAGGGAGCCCTTGGCCAGTGGTAAGTCCTGAGGC
AGGGGTTTGCGAGGCCTATCCTTCTCAACTCAACTAAGATGACCTCCCGCGTACCCGCATCAATACCA
ATACAACGTCCATGGCCCCCCCGGCTTTTACGGACACACCTGCACTTGTGTGCGGAACTTGTAACTTG
TAACTAACGAATGTACGGCCGCGCCACGTGCAAGAA**ACGCGT**TTTCCTTCCCGCACTTTTAGACCACA ***Mlu*I***
AGTTGCACACGTGTCAATTAGCAGCAGTGGTAGTAGGGATGAGTGTGCCTGATTGCTATGTCGCTAAT
AATACTCCTTCATGCCCCTGCTGTATCTTGCCTGCGCCCGTGCAGCTACGCCAGCATCTTCAACAGGG ***Kpn*I**
ACAACTCGGACTACTGCTGCCCCATCTACCGCACGGGGCCA**GGTACC**GGCGGAGGCGGTGGCATGAGC
AAGGGCGAGGAGCTGTTCACCGGCGTGGTGCCCATCCTGGTGGAGCTGGACGGCGACGTGAACGGCCA 5xG spacer
CAAGTTCAGCGTGAGCGGCGAGGGCGAGGGCGACGCCACCTACGGCAAGCTGACCCTGAAGCTGATCT
GCACCACCGGCAAGCTGCCCGTGCCCTGGCCCACCCTGGTGACCACCCTGGGCTACGGCCTGCAGTGC
TTCGCCCGCTACCCCGACCACATGAAGCAGCACGACTTCTTCAAGAGCGCCATGCCCGAGGGCTACGT mVenus
GCAGGAGCGCACCATCTTCTTCAAGGACGACGGTAACTACAAGACCCGCGCCGAGGTGAAGTTCGAGG coding
GCGACACCCTGGTGAACCGCATCGAGCTGAAGGGCATCGACTTCAAGGAGGACGGCAACATCCTGGGC sequence
CACAAGCTGGAGTACAACTACAACAGCCACAACGTGTACATCACCGCCGACAAGCAGAAGAACGGCAT
CAAGGCCAACTTCAAGATCCGCCACAACATCGAGGACGGCGGCGTGCAGCTGGCCGACCACTACCAGC
AGAACACCCCCATCGGCGACGGCCCCGTGCTGCTGCCCGACAACCACTACCTGAGCTACCAGAGCAAG
CTGAGCAAGGACCCCAACGAGAAGCGCGACCACATGGTGCTGCTGGAGTTCGTGACCGCCGCCGGCAT
CACCCTGGGCATGGACGAGCTGTACAAG**GGTACC**TGATTGCCGTAAGAGCAGTCATGGCGCTGGAGAG ***Kpn*I, stopp**
CGCAGCAGCCGGAAGTAGGGGTAGAAGTTGTTGTTGCTACAAGTGCAGCAGCAGGCAGAAGATAAGGA
GCACAATATGGCATCTTAGTACTGCATGAATGAACTGACATACAGACATGTTTACAGATCATCAGTCG
GCGGGTTTTTCACTTTATCTCTTCGTTCGGTTGCAGCAGTCGATAGATAGATAGACAGACGAGCTAGA
CAGTATGATTGATCTGTTGGACGGAATCTTTTCCTTTCCCCGACACAACTGCTTGTAGTAACATTTTT
TGTAATGATTT**ATCGAT**GTACCACAATTCCTCTCGAACAGTTACGAGGCTAGATACTCGGACAGGCCT ***Cla*I***

GGTAGGCAGGTGCTGCTGTGCTGCATATATCTATTAGGATGGTGGCGCAGAGGTTTCTTTGGTGGGTT
TGCATGTTGCCATAGACACCGCGGCCGGATGTGCACGGTTTATTAAATGATAATGTGGCTTGTGAAAT
TAACGCAAGTAGCTGGCGAGCAGTGGCTACTTGGTCAAGTGGACTGAGTCTGAGCATGACGTGGTGGG
ACGCGGTGCGGTCTATTTGGAGCACTAAAGTACATCTCGTCATCAGCAGGCTCTGCTGGGTCCTGCGG
GTGGCGCAAGTTTGAAACGAACGCGCGGTGGCACATTCTCGTGGGTGTCTTCACCAAGGAGTTCCAAA
TCCTAAGAACAAGGTTAGCCCAATGGAACTGCAGTGGCGTCTGAGGTAGCTGACGGTAGAGACAGATC
ACGGTGATACAGTAACCTTTTACCGGGGCACATTGTGGCGACTGGAGCCGCATGACCGTCCCCGTCAC
TTTGTAACCGCTCAAACTGCACGATAACTCCAACCCACACCGTCTTCAATGCGGCAGCTTGCGACGGT
TTCGC**<u>AGATCT</u>**TCCGAACTGCTCCAATAGCAGCTTGGGATCGACCCGTCATTTCTGCACCAAGTCGCA ***Bgl*II**
AAATAATGACAGATCCTAGGTGGCCGTGGTTATATGCTTTGCCACGTTGTAGAGTCCGAACTATATTG
TCTTCCCTATGGGCACCCATGGCCATGCTGGATGGCGAAGCACAGTGGTGAGCGGCCTAAGGTAGCTC
TCCGACCAGGAAAACATCACCAGTGCACAGCTCGTCATAGCGATGAATGTTGCAGGGGTGCAAAGGCA
TGTTCCACCACACCATTACGAGCAACCTTAGGACCGCGTTCCCCCAGGTAAACAGGGGAGGTTTCAGG
GGCTAGATATACTGGTCCAATAAGCAGGGTGCTATTGATGCAGGCGGTAATGTAGCACCCTCCCTCAT
CCGACGTACCTCACTCCCTGCACATGTAGAGCCCCTGCGTAGAACGGCTATCTGTGATGAGGGGGAGT
CCCTGGTATAGAGGCCAATCATGCAAACTCGCTGTGCAGTGCTTCATCAGTTAGGGAGCATGTGCCGT
TGTTGGACATTCGGGGACTGCGGGACAGCATTGTCAACATCGTTGCAGGCCCTGTAATGGGCCACATC
ATGCAGTAGGTTTCTAGCGGTTTCCGAGGCCGAGGTCATTTTGCCGGGGTGTACGGCATTGTTGCGGG
TTGCGGGAAGTTGTACAGGTAAATGCACCGGCCACATTTACCAACATTGCTTTAAATATAAGTAGACA
ACCGAGAAAGAACCAAAAGATGTCGGAAAGAATTTGGGCAGAGGCCGAAGCTCGCCTGGCAAGCACTG
CGCTGAACGGATAGAGAGAGACACGAATAAGAAGTGTACAACGGGGCCTCAATAGGCTTTGGGGTCCA
TAGATACCGGGCGCCCTCGCTCTCAGGCATTAAGTCTCGGACGCGGGCCACAAGACCTGGAGCTGCTT
GGCTGTTCCCTCTCGTCCCCCCCCTTCAGAAGAAAAACTCTGACCACTATCCCTCTCTCCAGTTCCCT
CTCAGTCTGGGTGGTGCAATACCAGACCCCTCGCCACACACACCGCCACCTCAGCACCAAACCGTCAC
ATTACGCTGCAAACATTGAGTCACGTTTGTTAGGCGCTAGCACGCTGTTGTATGAATTAGTTTCTGAG
TCTATGTTGATGTGGTTTGGTCCCGTTGCTGATGCAACTGGCTTTCGCATCATTAACCGCCGAGTAGC
AGCCGTAGCTACCGGTGCGGAAAACGATGCATGCTCACCAACCTAAATGATGAAGGGTGTGTGGCGAA
GTTATATTCATTATGCCAGGATCAGAGCTGTTGGTCAGTAAATATCAAGTTATATAAAAGAAATGGTG
CTACAGATTACAACGACGGGTCGGATTCCGACACGTACAACACGAGCAACATCCCAACGGATGAAATG
CACATTTATATGTGTCTGCGATTAAC**<u>GAATTC</u>** ***Eco*RI**

FIG. S3. **Genomic sequence of the *V. carteri phII* gene with *yfp* coding sequence added.** The sequence depicted here is present in plasmid pPhII-YFP. The chimeric gene consists of 8.3 kb genomic DNA including 5' and 3' regulatory sequences and the complete transcribed region of pherophorin II including all introns as present on scaffold 34. The *yfp* (mVenus) [S8] coding sequence was fused in frame with the coding sequence of the last *phII* exon and a 15 bp sequence coding for a pentaglycine flexible spacer. For the insertion of mVenus, artificial *Kpn*I sides were introduced by recombinant PCR which also allow for a later exchange of the fluorescent marker. The gene structure is indicated as follows: Coding sequences are shown with blue background, UTRs with green background and the promoter region with grey background. Start and stop codons are highlighted (violet font). The 5' UTR is just 14 bp in length, while there is a quite long 3' UTR of 1,168 bp. The coding sequence of mVenus is highlighted in yellow. The pentaglycine spacer is highlighted in orange. The restriction sites that are shown in SI Appendix, Fig. S1 A and B are marked (bold, underlined). Restriction sides that were used for inserting the *yfp* coding sequence are marked with asterisks.

## 2. SUPPLEMENTARY METHODS: SEMI-AUTOMATED IMAGE SEGMENTATION AND GEOMETRIC ANALYSIS

### A. Overview

We employ a semi-automated image analysis pipeline which uses Cellpose [S9] as a key step.

1. Contrast stretching of the image is performed by predetermined cutoffs, e.g. 2nd and 98th percentile intensity.

2. A J-invariant filtration is performed using (depending on the channel, fluorescence or trans-PMT) either (i) total-variation (TV) denoising by minimizing the Rudin-Osher-Fatemi functional

$$\min_{u \in \mathrm{BV}(\Omega)} \int_\Omega \left[ \|\nabla u\| + \frac{\lambda}{2}(f-u)^2 \right] \tag{S1}$$

   where $f$ is the intensity profile of an image supported on the image domain $\Omega$ to be denoised, or (ii) wavelet denoising with adaptive thresholding. A J-invariant filter is defined as one whose output value at every pixel is independent of the value of the source pixel (i.e. is only a function of source pixels at other locations). We find TV denoising in particular to be effective at filtering Poisson noise and significantly enhance the performance of Cellpose on low-SNR fluorescence images. We did not use the trained denoising model available in Cellpose3 [S10].

3. A user-prompted input polygon $P$ is used to estimate the diameter $d = \max\{\|\boldsymbol{v}_i - \boldsymbol{v}_j\| \mid \boldsymbol{v}_i, \boldsymbol{v}_j \in P\}$ of typical instances to be identified in the image, passed as the *diameter* input to the Cellpose *cyto3* model [S10].

4. Objects identified as pixel-space masks by Cellpose are converted to polygons in the plane by either (i) taking the convex hull, for convex objects such as somatic cells, or (ii) identifying outlines in the mask. Degenerate and invalid polygons are suppressed by taking a single binary erosion-dilation step. Further conversion to ellipses for approximately elliptical objects (such as parent and offspring spheroids) is performed by computing the ellipse with the same $n$th-order moments of area as the polygon (see §2 B) up to $n = 2$.

5. False-positives are manually rejected where identified. False-negatives, where identified, are re-prompted to Cellpose by restricting to a user-specified region of interest around the object, and re-iterating from step 1.

6. For identification of the somatic CZ3 geometry in particular, only the somatic cell-CZ3 compartment pairs (as seen in Fig. 5, main text) which have jointly been successfully identified are retained.

7. Downstream analysis of the resulting polygons and/or ellipses is performed as described in Table 1 (main text) and further detailed below in §2 B.

### B. Geometric moments of area

The geometric moments of bounded planar domains, analogous to the moments of bivariate uniform random variables, quantify shape properties such as size, center of mass, eccentricity, skew, and so on. In the case of polygonal domains, the geometric moments up to sufficiently high order completely determine the vertices [S11].

**Definition 2.1** (Planar $n$th area moment tensor)**.** Let $D \subset \mathbb{R}^2$ be an open measurable set with boundary given by a simple closed curve $\partial D = C$. The $n$th moment tensor for the domain $D$ of uniform mass density is

$$\mu_I^{(n)}(D) = \iint\limits_D \boldsymbol{x}^I d^2\boldsymbol{x} \tag{S2}$$

where $I = (i_1, \ldots, i_n)$ is a multi-index such that $i_j \in \{1, 2\}$ and

$$\boldsymbol{x}^I = \prod_{j=1}^{n} x_{i_j}. \tag{S3}$$

The 0th moment $\mu^{(0)}$ is the area of $D$. Accordingly, one may define the radius $R_D$ of an equivalent (same-area) circle as $R_D = \sqrt{\mu^{(0)}/\pi}$. The $n$th-order moments can be calculated for polygons by (i) applying the divergence theorem to write (S2) as a boundary integral on $C$, and (ii) computing the integral as a finite sum using the piecewise-linearity of the sides $C$.

### 1. *First moment and centrality*

**Definition 2.2** (Centroid)**.** The center of mass of $D$ is

$$\mu_j = \frac{\mu_j^{(1)}}{\mu^{(0)}}. \tag{S4}$$

The notation $\boldsymbol{\mu} = [\mu_1, \mu_2]$ evokes the probabilistic interpretation as the expected value of a uniform distribution supported on $D$. The basis in which (S2) is computed will unless otherwise specified be taken, for moments of order $\geq 2$, to be one in which $\boldsymbol{\mu}$ is at the origin.

**Definition 2.3** (Dimensionless centrality of a test point)**.** For a test point $\boldsymbol{y} \in \mathbb{R}^2$, we define the centrality metric

$$d_{\boldsymbol{\mu}}(\boldsymbol{y}) = \|\mathsf{W}(\boldsymbol{y} - \boldsymbol{\mu})\| = \sqrt{(\boldsymbol{y} - \boldsymbol{\mu}) \cdot \Sigma^{-1}(\boldsymbol{y} - \boldsymbol{\mu})} \tag{S5}$$

with $\mathsf{W}$ a matrix defined as $\mathsf{W}^\intercal \mathsf{W} = \Sigma^{-1}$, and $\Sigma$ the covariance matrix of $D$, defined in (S7).

This *whitening* procedure (again evoking the probabilistic interpretation of $\Sigma$) enables comparison across domains $D$ of varying second moment, resulting in a quantity which is dimensionless. In probability terms, (S5) is the Mahalanobis distance of $\boldsymbol{y}$ to the uniform distribution supported on $D$.

In particular, $d$ is scale-invariant; for dilations of space $\mathbb{R}^2 \mapsto \rho\mathbb{R}^2$, $\rho > 0$, we have $\boldsymbol{\mu} \mapsto \rho\boldsymbol{\mu}, \boldsymbol{y} \mapsto \rho\boldsymbol{y}$, and $\Sigma \mapsto \rho^2\Sigma$ by (S7), hence $d_{\boldsymbol{\mu}}(\boldsymbol{y}) \mapsto d_{\boldsymbol{\mu}}(\boldsymbol{y})$ by (S5). Moreover, dilations preserve aspect ratios, since

$$\Sigma \overset{\mathbb{R}^2 \mapsto \rho\mathbb{R}^2}{\mapsto} \frac{1}{\rho^2 |D|} \iint\limits_D \rho(\boldsymbol{x} - \boldsymbol{x'}) \otimes \rho(\boldsymbol{x} - \boldsymbol{x'}) \rho^2 d^2\boldsymbol{x'} = \rho^2 \Sigma, \tag{S6}$$

hence its eigenvalues map as $\lambda_j \mapsto \rho^2 \lambda_j$ and the ratio $\lambda_{\max}/\lambda_{\min}$ is preserved.

### 2. *Second moment and isotropy*

**Definition 2.4** (Covariance matrix of a domain)**.** The normalized second central moment, or covariance matrix, is

$$\Sigma = \frac{\mu^{(2)}}{\mu^{(0)}} \tag{S7}$$

As before, *central* indicates that $\mu^{(2)}$ is computed in a basis in which $\boldsymbol{\mu}$ is at the origin.

In probability terms, $\Sigma$ is the covariance matrix of a uniform distribution supported on the domain $D$. If $D$ has radial symmetry about $\boldsymbol{\mu}$ (either continuous, as a circle does, or discrete, as regular $n$-gons do), then $\Sigma = c\mathsf{I}$ for some $c > 0$. This is verified by the existence of an eigenspace of dimension 2. $\Sigma^{-1} = \mathsf{M}$ is the matrix defining an ellipse with the same aspect ratio as $D$.

**Definition 2.5** (Principal axes of a domain)**.** Using (S7), we may define the principal axes and stretches of a domain $D$ via Hermitian eigendecomposition

$$\Sigma = \mathsf{P}\Lambda\mathsf{P}^{-1} \tag{S8}$$

with $\boldsymbol{v}_i$ the columns of $\mathsf{P}$ being the principal axes and and $\lambda_i > 0$ in ascending order (as $\Sigma$ is symmetric positive-definite for non-degenerate curves).

**Definition 2.6** (Aspect ratio of a domain)**.** Let $\lambda_1, \lambda_2$ and $v_1, v_2$ be the principal stretches and axes (in ascending order) of $\Sigma$ as in (S8). The aspect ratio is

$$\alpha = \sqrt{\frac{\lambda_2}{\lambda_1}}. \tag{S9}$$

Ellipses (objects defined uniquely by their moments to order $n = 2$) with the same orientation, aspect ratio, and area ($\pi ab$) as $D$ have the minor and major axes

$$a = \sqrt{\frac{\mu^{(0)}}{\pi\alpha}}, \quad b = \alpha a. \tag{S10}$$

Equation (S10) is an exact elliptical representation of a polygon (or arbitrary domain), in contrast to elliptical approximations, e.g. (i) weighted $\ell^2$-minimization of vertex distance or (ii) convex programs for minimum-area bounding ellipses.

### 3. *Moments under affine transforms*

Let $\mathsf{F} > 0$ be a symmetric positive-definite matrix (e.g. a strain tensor) and define an affine transform of a domain $D$ about its center of mass by

$$T(\boldsymbol{x}) = \mathsf{F}(\boldsymbol{x} - \boldsymbol{\mu}) + \boldsymbol{\mu}. \tag{S11}$$

Let $T(D)$ be the transformed region. By change of coordinates for integrals, the relevant moments of $T(D)$ are

$$\mu^{(0)}(T(D)) = \iint_{T(D)} d^2\boldsymbol{y} = \iint_{D} \det \mathsf{F} d^2\boldsymbol{x} = \mu^{(0)}(D) \det \mathsf{F} \tag{S12}$$

$$\mu^{(1)}(T(D)) = \iint_{T(D)} y d^2\boldsymbol{y} = \iint_{D} (\mathsf{F}(\boldsymbol{x} - \boldsymbol{\mu}) + \boldsymbol{\mu}) \det \mathsf{F} d^2\boldsymbol{x} = \mu^{(1)}(D) \det \mathsf{F} \tag{S13}$$

$$\boldsymbol{\mu}(T(D)) = \mu^{(1)}(T(D))/\mu^{(0)}(T(D)) = \boldsymbol{\mu}(D) \tag{S14}$$

$$\mu^{(2)}(T(D)) = \iint_{T(D)} (\boldsymbol{y} - \boldsymbol{\mu}) \otimes (\boldsymbol{y} - \boldsymbol{\mu}) d^2\boldsymbol{y} = \iint_{D} \mathsf{F}(\boldsymbol{x} - \boldsymbol{\mu}) \otimes \mathsf{F}(\boldsymbol{x} - \boldsymbol{\mu}) \det \mathsf{F} d^2\boldsymbol{x} = \mathsf{F}\mu^{(2)}(D)\mathsf{F}^{\mathsf{T}} \det \mathsf{F} \tag{S15}$$

$$\Sigma_{T(D)} = \mu^{(2)}(T(D))/\mu^{(0)}(T(D)) = \mathsf{F}\Sigma_D\mathsf{F}^{\mathsf{T}} \tag{S16}$$

hence the centroid is preserved and the covariance matrix maps as $\Sigma \mapsto \mathsf{F}\Sigma\mathsf{F}^{\mathsf{T}}$.

### 4. *Whitening a domain*

Let a domain $D$ have covariance matrix $\Sigma$ (S7). Define the *whitened* domain $D_W$ by the affine transform $T$ as defined in (S11),

$$D_W = \{T(\boldsymbol{x}) \mid \boldsymbol{x} \in D\}, \quad \mathsf{F} = \Sigma^{-1/2}, \tag{S17}$$

with the matrix square root $\mathsf{F}$ typically approximated by singular value decomposition (SVD) as

$$\mathsf{F} \overset{\varepsilon \to 0^+}{=} \mathsf{U}(\mathsf{S} + \varepsilon)^{-1/2}\mathsf{U}^*, \quad \Sigma = \mathsf{U}\mathsf{S}\mathsf{V}^{\mathsf{T}}, \tag{S18}$$

and $\mathsf{F}$ the *ZCA whitening matrix* [S12] with regularization constant $\varepsilon \ll 1$. Then $D_W$ has aspect ratio 1 as defined in (S9).

## C. Isoperimetric problems

We recall here several quantities which can be used as measures of the deviation of a domain $D$ from a disk.

### 1. *Classical isoperimetric inequalities*

One has

$$4\pi A \leq L^2, \tag{S19}$$

where $A$ is the area of $D$ and $L$ the total arclength of $C$ (which we may now require to be a rectifiable Jordan curve) and is an equality only for circles. Accordingly, one defines an *isoperimetric quotient*, which we term the *circularity* in the main text,

$$q = \frac{\sqrt{4\pi A}}{L} \in [0,1], \tag{S20}$$

maximized for disks. For regular $n$-gons, one has

$$q_n = \sqrt{\frac{\pi}{n}\cot\frac{\pi}{n}}. \tag{S21}$$

A natural question is whether (S19) can be used to define a set distance, in the sense of Hausdorff metric, of $D$ to the "best" disk. This turns out [S13] to be related to the problem of making (S19) *quantitative*, in the sense of a nonnegative quantity $\nu(D)$ such that

$$4\pi A + \nu(D) \leq L^2 \tag{S22}$$

for all $D$, with $\nu(D) = 0$ iff $D$ is a disk. Without proof, we cite [S13] the result that the *isoperimetric deficit*, defined as the dimensionless quantity

$$\mathrm{ID}(D) = \frac{1-q}{q} \tag{S23}$$

upper-bounds any such quantitative inequality $\nu(D)$ via

$$\nu(D) \leq C_2\sqrt{\mathrm{ID}(D)} \tag{S24}$$

for some dimension-dependent constant $C_2$. For convex $D$ (applicable e.g. to the cells of a Voronoi tessellation), (S23) upper-bounds the Hausdorff distance $d_H$ to the best-fit equal-volume ball $B$ as

$$\inf_{\boldsymbol{x}\in\mathbb{R}^2} d_H(D, B+\boldsymbol{x}) \leq C_2 \mathrm{ID}(D)^{\alpha_2} \tag{S25}$$

for dimension-dependent constants $C_2, \alpha_2$ [S13]. Equality is achieved for $D$ which is a ball.

### 2. *Weighted isoperimetric inequalities*

Recalling the second moment $M_2$ as defined in the main text, eq. 1, written here with explicit arguments $M_2(\boldsymbol{x}, D)$, we recall by classical results that its minimization is also an isoperimetric problem.

**Lemma 1** (Disks minimize $\mathrm{Tr}(M_2)$)**.** Let $D \subset \mathbb{R}^2$ be as in Definition 2.1, $|D|$ its Lebesgue measure, and $\boldsymbol{x} \in \mathbb{R}^2$. We have $\mathrm{Tr}(M_2(\boldsymbol{x}, D)) \geq \frac{|D|^2}{2\pi}$ with equality iff $D$ is a disk and $\boldsymbol{x}$ is its centroid.

*Proof.* Write $\mathrm{Tr}(M_2)$ as

$$U(\boldsymbol{x}, D) = \mathrm{Tr}(M_2(\boldsymbol{x}, D)) = \iint_D \mathrm{Tr}[(\boldsymbol{x'}-\boldsymbol{x})\otimes(\boldsymbol{x'}-\boldsymbol{x})]d^2\boldsymbol{x'} = \iint_D \|\boldsymbol{x'}-\boldsymbol{x}\|^2 d^2\boldsymbol{x'}. \tag{S26}$$

Then optimality in the first argument implies

$$0 = \frac{\partial U}{\partial \boldsymbol{x}} = 2 \iint\limits_D (\boldsymbol{x'} - \boldsymbol{x}) d^2\boldsymbol{x'}, \tag{S27}$$

which holds iff $\boldsymbol{x} = \boldsymbol{\mu}$ is the centroid of $D$. Locating $\boldsymbol{\mu}$ at the origin without loss of generality, we have

$$U(\boldsymbol{x}, D) \geq U(\boldsymbol{\mu}, D) = \iint\limits_D |\boldsymbol{x'}|^2 \, d^2\boldsymbol{x'}. \tag{S28}$$

Recognizing the last expression as the polar moment of inertia and applying a *weighted* isoperimetric inequality (7.2, [S14]),

$$\geq \iint\limits_{B_{R_D}(0)} |\boldsymbol{x'}|^2 \, d^2\boldsymbol{x'}, \tag{S29}$$

where $B_{R_D}(0)$ is a disk at the origin of the same area as $D$ (i.e. $R_D$ is $D$'s circular radius as in §B). Thus

$$= \frac{\pi R_D^4}{2} = \frac{|D|^2}{2\pi}. \tag{S30}$$

□

Recall also the (standardized) sum of second moments, Eq. 3, main text. Using the previous lemma we may establish the following optimality for it in terms of honeycombs.

**Lemma 2** (Second moment bound for tessellations)**.** For any space packing $\{\boldsymbol{x}_i\}_{i=1}^n, \{D_i\}_{i=1}^n$ with standardized sum of second moments $m_2$ defined as

$$m_2 = n \sum_{i=1}^n \mathrm{Tr}(\mathsf{M}_2^{(i)}(\boldsymbol{x}_i, D)) / \left( \sum_{i=1}^n |D_i| \right)^2, \tag{S31}$$

we have $m_2 \geq \frac{1}{2\pi}$.

*Proof.* Let $A = \sum_{i=1}^n |D_i|$ and $\mathsf{M}_2(\boldsymbol{x}_i, D_i) = \mathsf{M}_2^{(i)}$. Then

$$m_2 = \frac{n}{A^2} \sum_{i=1}^n \mathrm{Tr}\, \mathsf{M}_2^{(i)} \tag{S32}$$

$$\overset{\text{CS}}{\geq} \frac{1}{A^2} \left( \sum_{i=1}^n (\mathrm{Tr}\, \mathsf{M}_2^{(i)})^{1/2} \right)^2 \tag{S33}$$

$$\overset{\text{L1}}{\geq} \frac{1}{A^2} \left( \sum_{i=1}^n \frac{|D_i|}{\sqrt{2\pi}} \right)^2 \tag{S34}$$

$$= \frac{1}{2\pi}, \tag{S35}$$

where the first inequality is Cauchy-Schwarz and the second is Lemma 1. □

Note that the first inequality is sharp only for configurations consisting of congruent cells $D_i$. The second inequality cannot be sharp for space *partitions*, only *packings* consisting of congruent disks. Space *partitions* optimize the second only if they are asymptotically (in $n$) regular hexagonal lattices [S15, S16].

### D. Average number of neighbors in a spherical Voronoi tessellation

Let $\{\boldsymbol{x}_i\}_{i=1}^n$ be a collection of points on the surface of a sphere and $\{V_i\}_{i=1}^n$ the corresponding set of spherical polygons given by their Voronoi tessellation. The number of neighbors of each $V_i$ is precisely the degree (number of

incident edges) $d(\boldsymbol{x}_i)$ of each node in the topological dual, the Delaunay triangulation $\{T_j\}_{j=1}^{f}$ of $\{\boldsymbol{x}_i\}$. Let $m$ be the number of edges; since this is a triangulation of a compact (boundaryless) surface, we have the relation $3f = 2m$. By the Euler theorem,

$$n - m + f = \chi = 2 \tag{S36}$$

where $\chi$ is the Euler characteristic of the sphere. Substituting the triangulation property into (S36) yields $m = 3n-6$, hence the average degree $\overline{d}$ is

$$\overline{d} = \frac{1}{n}\sum_{i=1}^{n} d(\boldsymbol{x}_i) = \frac{2m}{n} = \frac{6n-12}{n} \xrightarrow{n\to\infty} 6, \tag{S37}$$

thus the average number of neighbors of a Voronoi polygon is asymptotically 6.

## 3. SUPPLEMENTARY ANALYSES

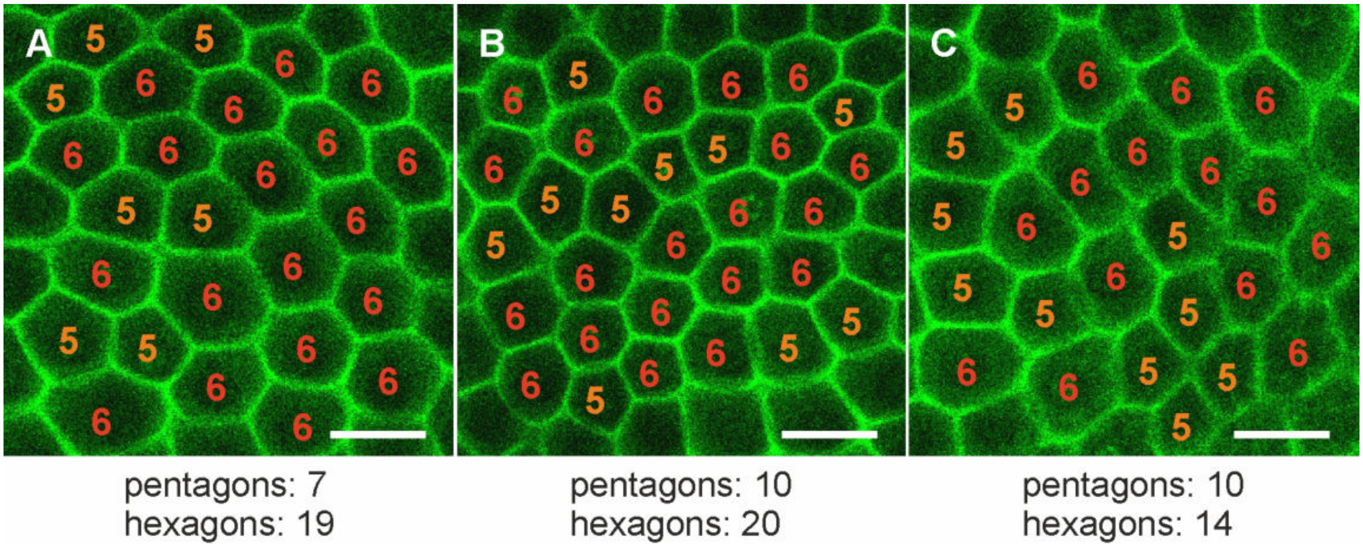


FIG. S4. **Share of pentagonal and hexagonal somatic CZ3 compartments in middle aged adults (early stage II).** Sexually induced transformants expressing the *phII:yfp* gene under the control of the endogenous *phII* promoter were analyzed in vivo for the localization of the PHII:YFP fusion protein. Magnified view of the PhII:YFP-stained compartments surrounding the somatic cells corresponding to CZ3. In areas where no gonidia lie below the somatic cell sheet, the compartments form a pattern of hexagons and pentagons. In the exemplary regions shown here, 27 pentagonal and 53 hexagonal compartments were counted, representing a ratio of roughly 1:2. Scale bars are 20 $\mu$m.

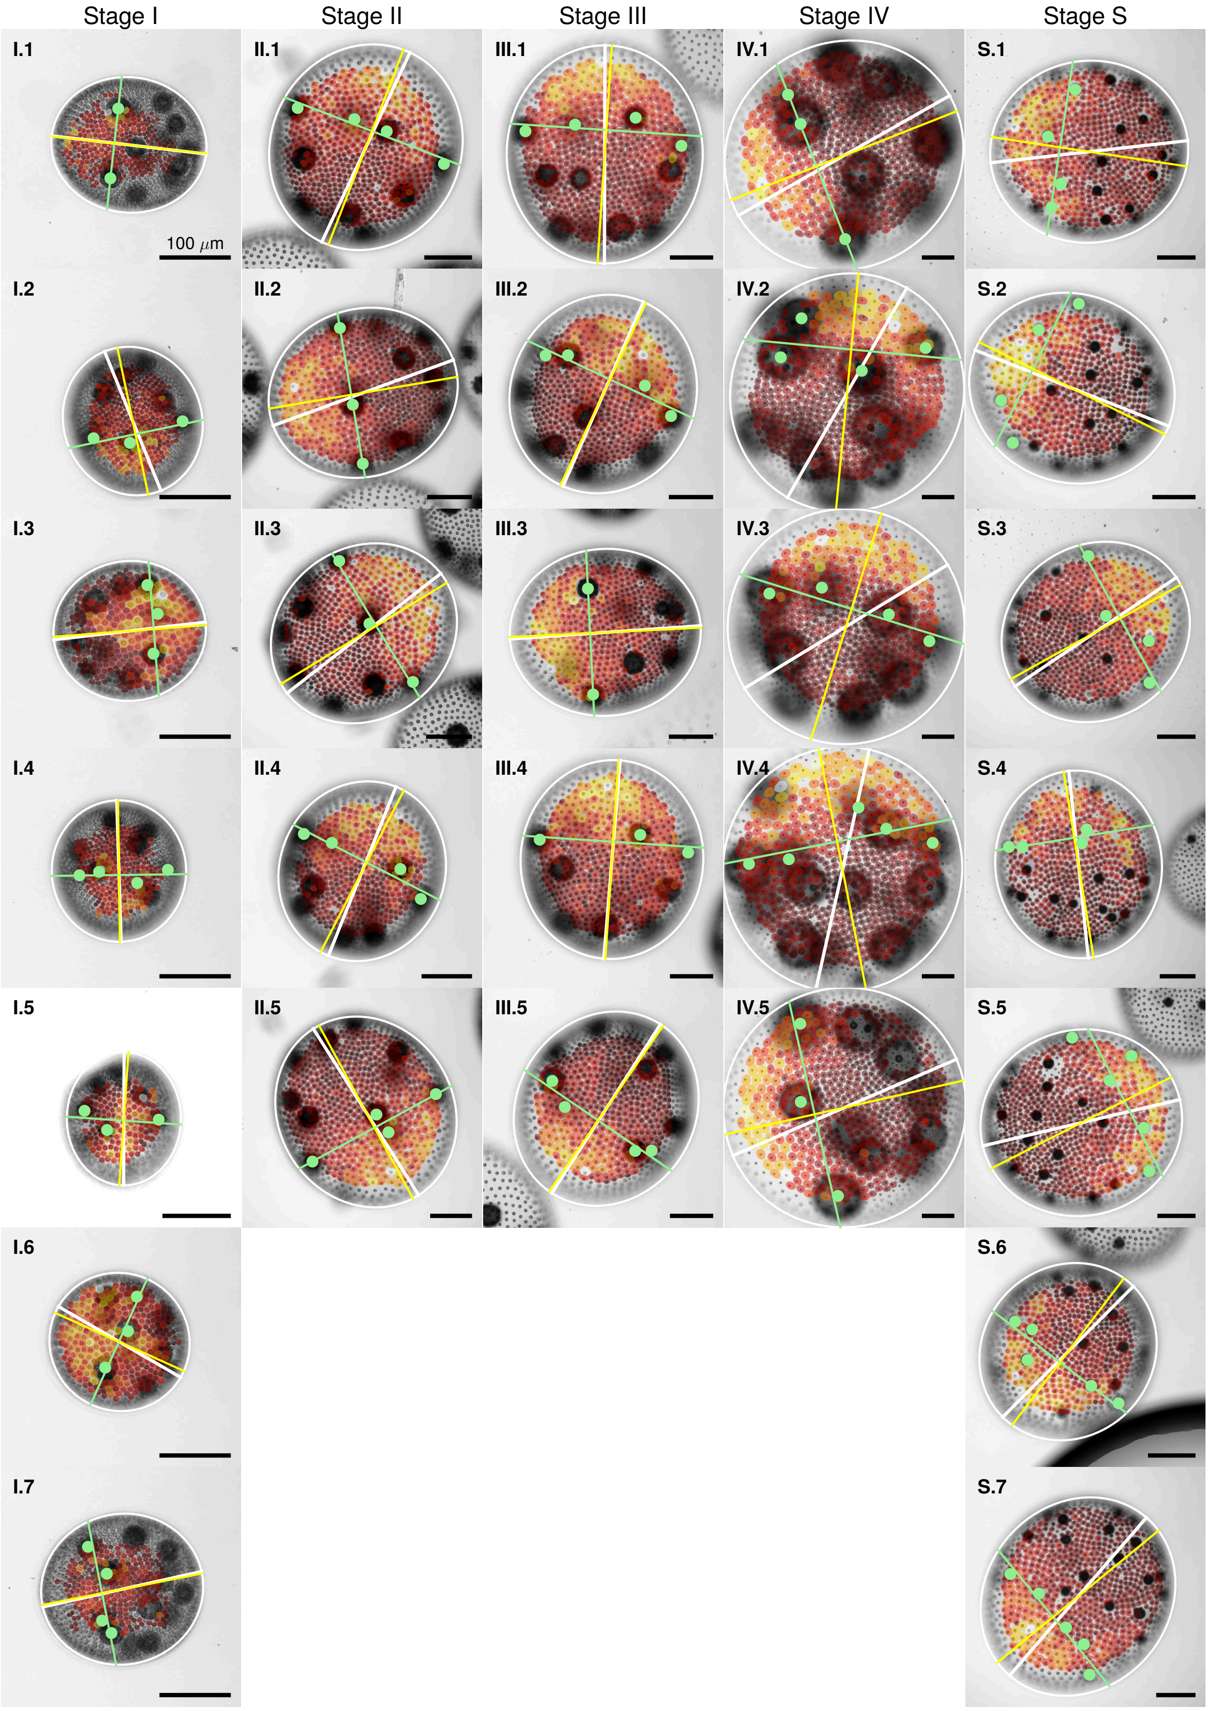


FIG. S5. **Segmented PhII:YFP signal and anterior-posterior axis identification.** Trans-PMT images of spheroid in stage I-IV and S (defined in Fig. 3 in the main document) with posterior-anterior axis (yellow line) estimated as the line passing through the elliptical (white outline) center which is normal to the best-fit line (green) through manually identified offspring (green dots) located in the anterior section. The white line represents the major axis of the ellipsoid. Overlaid are segmentations of the CZ3 compartments (PhII:YFP), colored by area (dark to light by size).

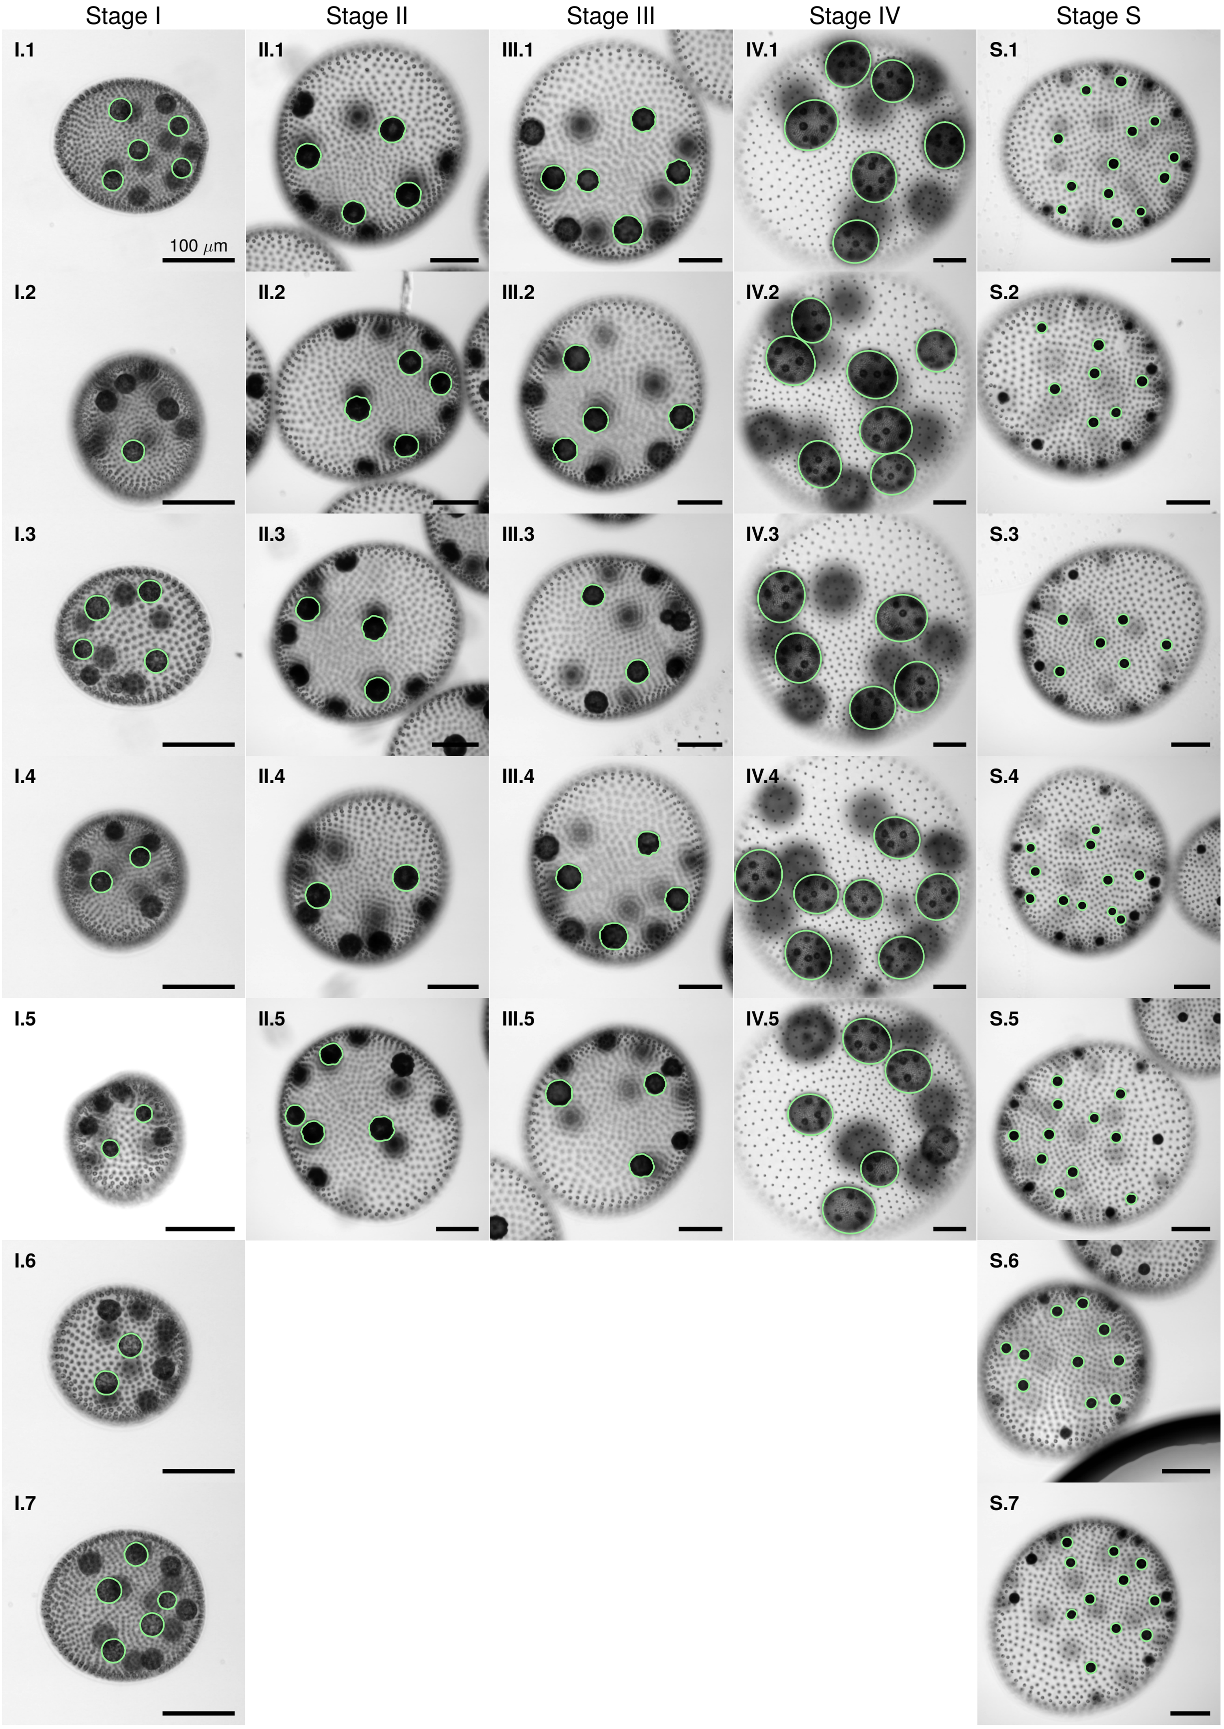


FIG. S6. **Offspring.** Offspring are identified using the same semi-automated procedure as that used for identification of somatic cells and CZ3 compartment geometry. Being far larger than either of those, however, offspring appear in focus at different planes. We identify offspring from planes where clearly in focus, displaying here particular planes for each spheroid. The boundaries are used to estimate the volumetric growth rates displayed in Table 2, main text.

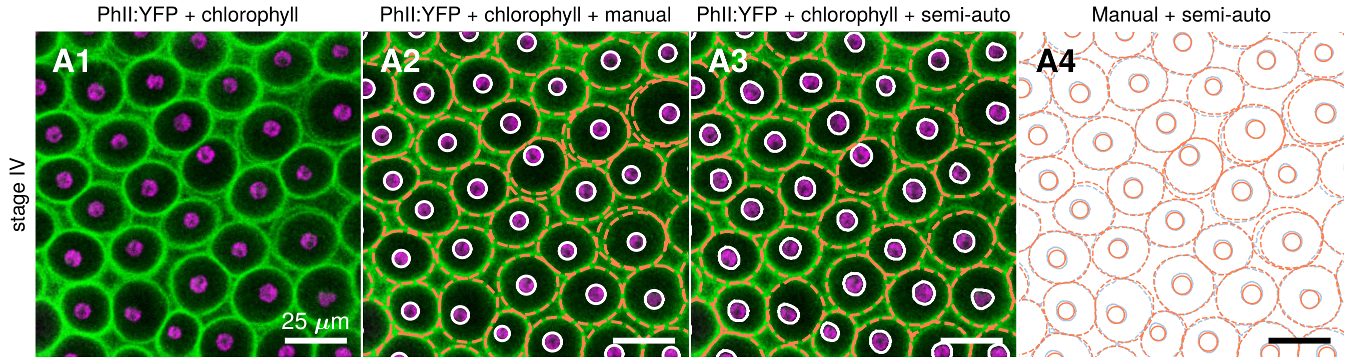


FIG. S7. **Comparison of semi-automated segmentation against fully manual segmentation.** 1. Overlay of YFP fluorescence of PhII:YFP protein (green) and chlorophyll fluorescence (magenta), detected at 650-700 nm. 2. Same as 1 with *manually* segmented CZ3 (orange) and cell boundaries (white), identical to panel A2, Fig. 5 in the main text. 3. Same as 2 with *semi-automatically* segmented (using the procedure described in §2) CZ3 (orange) and cell boundaries (white). 4. Comparison of semi-automated segmentation (blue, CZ3 compartments and cells) with fully manual segmentation (orange, CZ3 compartments and cells).

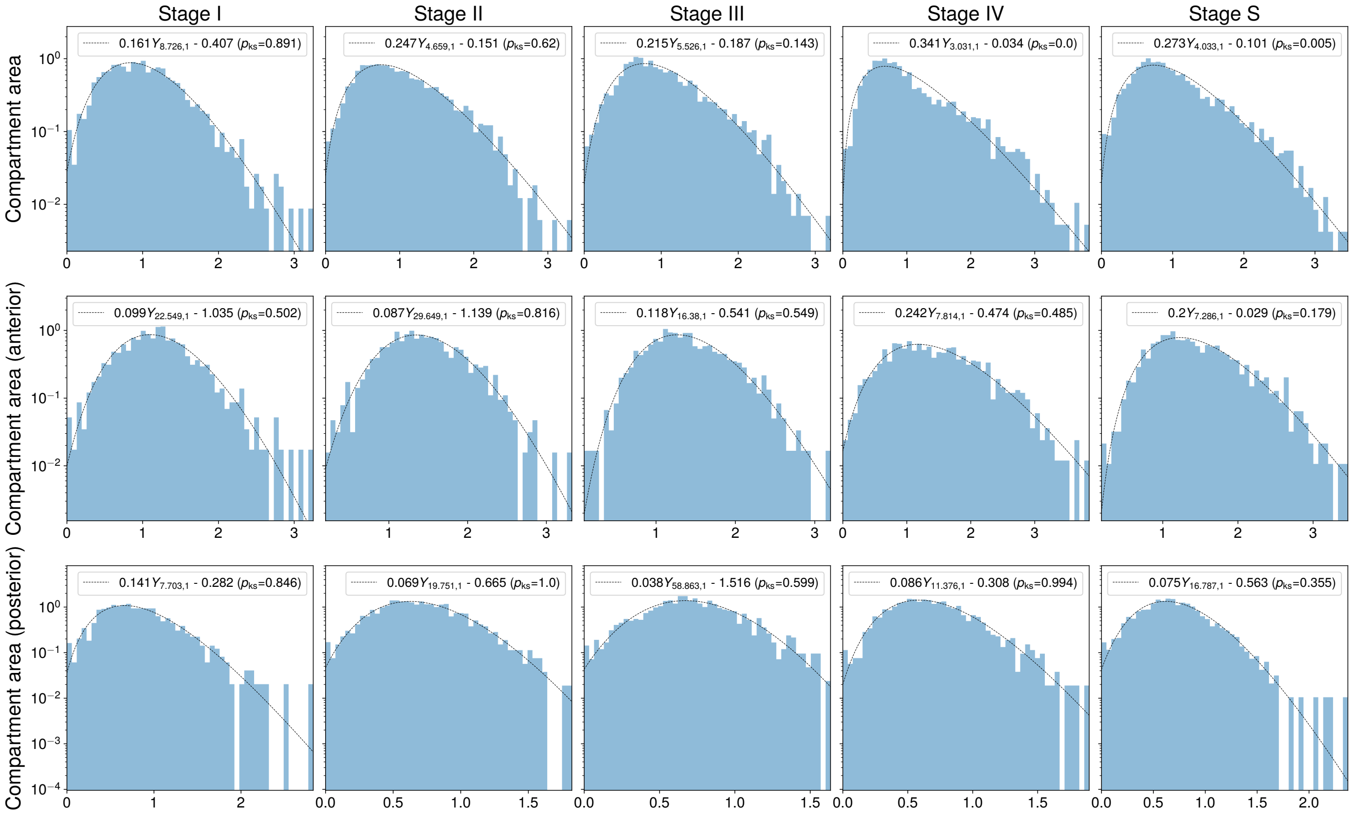


FIG. S8. **Areas are gamma-distributed throughout growth with changing shape parameters reflecting anterior-posterior differentiation.** Areas of CZ3 compartments robustly follow gamma-distributions, as highlighted in Fig. 8B2 and §E, main text. Plotted on y-axes (shared by row) are normalized counts per bin ($n = 50$ bins), and on x-axes are the reduced CZ3 areas $\tilde{a}_{\mathrm{cz3}} = (a_{\mathrm{cz3}} - a_{\min})/(a_{\mathrm{avg}} - a_{\min})$, where $a_{\min}$ and $a_{\mathrm{avg}}$ are minimum and average values of $a_{\mathrm{cz3}}$ for the respective spheroid. Such normalization enables distributional fit across different organisms. The empirical mean is therefore fixed at 1 in these distributions, and the maximum-likelihood fit parameters are $k$ and offset of the support (with $\lambda$ determined by the relation between $k$ and the fixed mean). A Kolmogorov-Smirnov (KS) goodness-of-fit test is performed and its $p$-value is recorded as $p_{\mathrm{ks}}$ in each plot. One key observation we make, evident in the first row, is that the extreme degree of anterior-posterior differentiation (shown in Fig. 8B1, main text) suggests that a single fit from this distribution family may not be valid in later stages of the life cycle. Indeed, $p_{\mathrm{ks}} \approx 0.9$ in stage I, indicating no strong evidence that $\tilde{a}_{\mathrm{cz3}}$ do not arise from a gamma distribution, yet drops below 0.001 by stage IV, supporting rejection of the fit hypothesis in this case. Qualitatively, one observes the formation of "shoulders" in the distribution (exhibiting a loss of log-concavity which does not hold in the gamma distribution for shape parameter $k \geq 1$). Separating the data by anterior/posterior hemispheres, however, almost completely resolves the issue and reveals that the respective $\tilde{a}_{\mathrm{cz3}}$ values follow gamma distributions (of very different shape parameters). Lastly, fitted parameters of the sexual stage S place it distributionally closer to Stage IV than to III, which contrasts with the grouping inferred from the spheroid radii (Fig. 10E, main text).

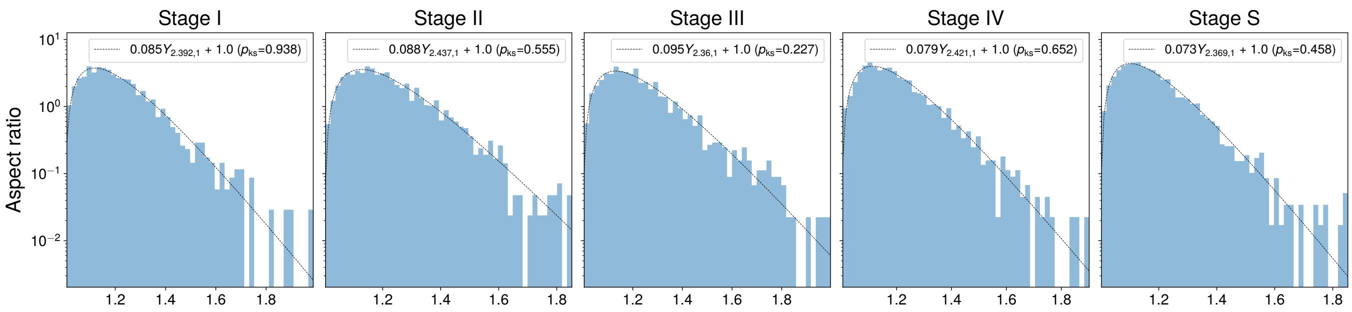


FIG. S9. **Aspect ratios remain stably gamma-distributed throughout growth.** As seen, the $k$ parameter remains in a remarkably tight range between $2.35 - 2.45$. Maximum-likelihood estimated (MLE) parameters include only rate $\lambda$ and shape $k$, with location fixed at 1. Both this distribution family and the value of the shape parameter for aspect ratios are robustly observed in a variety of living organisms and inert jammed systems [S17]. Kolmogorov-Smirnov tests performed in each case indicate no strong evidence that the data do not follow gamma distributions.

| Stage | Spheroid volume change (est., mm$^3$) | Total offspring volume change (est., mm$^3$) | Total cell volume change (est., $\mu$m$^3$) | % spheroid volume change to offspring (est., %) | % spheroid volume change to cells (est., %) | Elapsed time (h) | Spheroid growth rate (est., mm$^3$/h) | Total offspring volume growth rate (est., mm$^3$/h) | Total cell volume growth rate (est., $\mu$m$^3$/h) |
|---|---|---|---|---|---|---|---|---|---|
| I | ↓ | ↓ | ↓ | ↓ | ↓ | ↓ | ↓ | ↓ | ↓ |
| II | 0.040 | 0.0011 | $2.9 \times 10^5$ | 2.8 | 0.73 | 15 | 0.0027 | $7.5 \times 10^{-5}$ | 9.8 |
| III | 0.015 | 0.00019 | $1.9 \times 10^4$ | 1.2 | 0.13 | 6 | 0.0025 | $3.1 \times 10^{-5}$ | 1.6 |
| IV | 0.26 | 0.026 | $9.4 \times 10^4$ | 10 | 0.037 | 16 | 0.016 | 0.0016 | 2.9 |

TABLE S1. Estimated volumetric growth changes by life cycle stage (I-IV), supplementary to Table 2, main text. Number of juveniles per spheroid were manually estimated from the trans-PMT image (as in Fig. S6), with the average value over all $n = 29$ spheroids being exactly 13. The estimated total offspring volume change (column 3) is defined as this number, times the average estimated juvenile volume per stage (as given in Table 2, main text, computed from segmentation of the trans-PMT image, Fig. S6). Further, assuming a fixed count of $2^{11} \approx 2000$ somatic cells per spheroid and multiplying this times the average somatic cell volume per stage (again Table 2, main text) yields the estimated total volume change due to somatic cells (column 4). Assuming $2^{12}$ somatic cells changes the contribution to the overall spheroid volume negligibly, as evident from column 6. Taken together, columns 2, 3, and 4 yield an estimation of the contribution to overall spheroid volume change by offspring, somatic cells, and parental ECM (Table 2, column 5, main text) by subtracting columns 3 and 4 from 2. Lastly, knowledge of the approximate elapsed time between life cycle stages (column 7) yield the corresponding estimated growth rates (columns 8-10 here and Table 2, columns 5-6, main text).

| | Cell area | Compartment area | Aspect ratio | Circularity | Offset | Offset (whitened) | Voronoi error |
|---|---|---|---|---|---|---|---|
| % change PA in stage I | 14 | 44 | 9.8 | −2.5 | 47 | 23 | 1.7 |
| % change PA in stage II | 13 | 94 | 3.1 | −0.69 | 120 | 65 | 16 |
| % change PA in stage III | 13 | 120 | 1.0 | −0.67 | 82 | 37 | −6.6 |
| % change PA in stage IV | 8.1 | 130 | 14 | −0.53 | 50 | 8.7 | −10 |
| % change PA in stage S | 9.9 | 130 | −1.8 | −1.9 | 200 | 110 | −3.1 |
| Mean value in stage I | 26 $\mu$m | 58 $\mu$m$^2$ | 1.2 | 0.88 | 0.54 $\mu$m | 0.24 | 0.21 |
| % change stages I to II | 81 | 200 | 0.93 | 1.9 | 140 | 43 | 22 |
| Abs. change stages I to II | 21 | 120 | 0.011 | 0.017 | 0.76 | 0.11 | 0.045 |
| % change stages II to III | 2.4 | 30 | 0.86 | −0.78 | 27 | 12 | −1.4 |
| Abs. change stages II to III | 1.1 | 52 | 0.010 | −0.070 | 0.35 | 0.042 | −0.036 |
| % change stages III to IV | 12 | 170 | −2.7 | 1.8 | 53 | −5.6 | 16 |
| Abs. change stages III to IV | 6.0 | 370 | −0.34 | 0.016 | 0.87 | −0.22 | 0.039 |

TABLE S2. Summary of changes in mean value along posterior-anterior axis (PA) and by life cycle stage (I-IV, S). Rows 1-5 show the changes in empirical mean value from posterior to anterior end within each life cycle stage. Rows 6-12 show the changes in mean value across successive life cycle stages. While the underlying distributions are highly skewed and mean-based comparisons should be interpreted carefully as noted in §E1 (main text), they provide one quantification of the underlying trends visible in the empirical distributions, Fig. 8, main text.

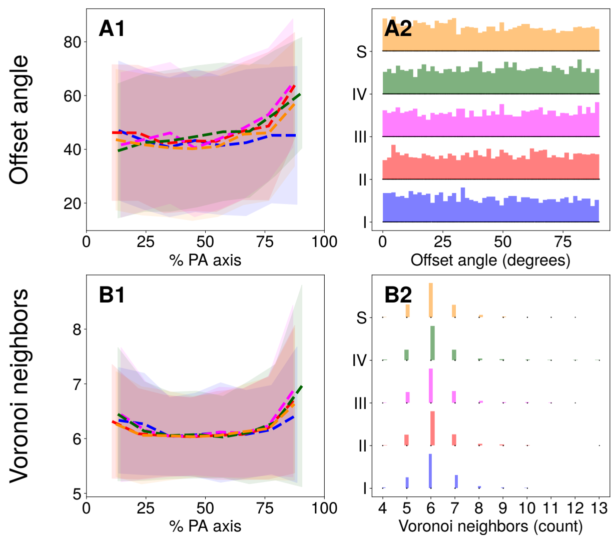


FIG. S10. **Additional invariances in the stochastic geometry of the CZ3 compartments across the life cycle.** Rows A and B follow the same formatting as Fig. 8, main text. Row A shows variation in the offset angle $\theta_{\mathrm{cell}} = \arccos(|\Delta\boldsymbol{x} \cdot \boldsymbol{v}| / (\|\Delta\boldsymbol{x}\| \, \|\boldsymbol{v}\|))$ between the somatic cell offset vector $\Delta\boldsymbol{x}$ (Table 1, main text) and the principal stretch axis $\boldsymbol{v}$ of the CZ3 compartment (given by the eigenvector corresponding to $\lambda_{\max}$). Since the latter has no polarity, $\theta_{\mathrm{cell}} \in [0, 90]$ degrees. Panel A1 shows that there is little variation along the PA axis or by life cycle, with the exception of upward tails toward the anterior pole in stages II-IV and S. Panel A2 reveals furthermore that $\theta_{\mathrm{cell}}$ effectively follows a uniform distribution over its support throughout the lifcycle, indicating that there is no correlation between the somatic cell offset vector $\Delta\boldsymbol{x}$ and the principal stretch axis. This is perhaps surprising given that one might naively expect translation of the cell along the deformation axis of its compartment. Row B shows, in the same format, the number of neighbors (edges) of each Voronoi partition. Panel B1 again shows that there is almost no variation along the PA axis or by life cycle stage, providing quantitative evidence that the topology of the CZ3 space partition does not change during growth. Panel B2 displays the distribution of Voronoi neighbors by life cycle stage, whose mean is around 6, consistent with Euler's theorem for Voronoi tessellations of the sphere (§2 D).

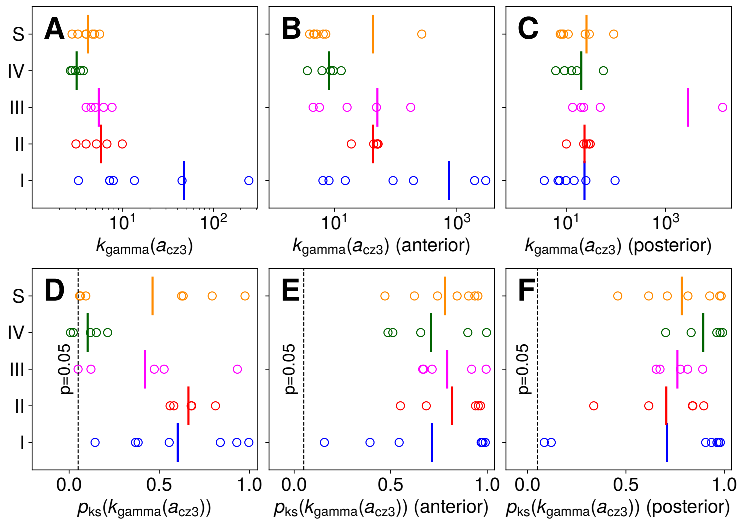


FIG. S11. **Increasing area polydispersity during the life cycle is primarily due to changes in the anterior hemisphere.** Panel A is the same as Fig. 10B (main text) while panels B and C show the same metrics separated by anterior and posterior regions respectively. As seen, B shows a decrease in $k$ (in increase in disorderedness as explained in main text) of the anterior configuration by life cycle stage, while C shows relatively stable values in the posterior configuration. The former therefore likely underlies the increasing disorderedness observed in the whole spheroid (panel A). Panels D-F display the respective $p$-values ($p_{\mathrm{ks}}$) of a Kolmogorov-Smirnov goodness-of-fit test performed in each instance of the $k_{\mathrm{gamma}}$ value reported in panels A-C. All panels D-F show that stage I can exhibit varying degrees of goodness-of-fit, which is likely reflected by the large spread of $k$-values in stage I (panels A-C). However, in the progression from stages II-IV and S, $p_{\mathrm{ks}}$ drops significantly, sometimes below the threshold (plotted as dashed vertical lines), as expected from Fig. S8, despite the qualitatively good match observed in row 1 of that figure. As in Fig. S8 rows 2-3, this is remedied by separating into anterior/posterior hemispheres, at which point the data collapses well, indicated by the sharp increases in $p_{\mathrm{ks}}$ in panels E-F. Remarkably, this increase in goodness-of-fit accompanies a clear observation in panels B-C that the anterior hemisphere is primarily responsible for increasing disorder in the somatic CZ3 configuration.

## SI REFERENCES


[S1] B. von der Heyde and A. Hallmann, Targeted migration of pherophorin-S indicates extensive extracellular matrix dynamics in *Volvox carteri*, The Plant Journal **103**, 2301 (2020).

[S2] S. E. Prochnik, J. Umen, A. M. Nedelcu, A. Hallmann, S. M. Miller, I. Nishii, P. Ferris, A. Kuo, T. Mitros, L. K. Fritz-Laylin, *et al.*, Genomic analysis of organismal complexity in the multicellular green alga *Volvox carteri*, Science **329**, 223 (2010).

[S3] D. M. Goodstein, S. Shu, R. Howson, R. Neupane, R. D. Hayes, J. Fazo, T. Mitros, W. Dirks, U. Hellsten, N. Putnam, *et al.*, Phytozome: a comparative platform for green plant genomics, Nucleic acids research **40**, D1178 (2012).

[S4] B. Klein, D. Wibberg, and A. Hallmann, Whole transcriptome RNA-Seq analysis reveals extensive cell type-specific compartmentalization in *Volvox carteri*, BMC Biol. **15**, 111 (2017).

[S5] A. Hallmann, Extracellular matrix and sex-inducing pheromone in *Volvox*, International Review of Cytology **227**, 131 (2003).

[S6] S. El-Gebali, J. Mistry, A. Bateman, S. R. Eddy, A. Luciani, S. C. Potter, M. Qureshi, L. J. Richardson, G. A. Salazar, A. Smart, *et al.*, The pfam protein families database in 2019, Nucleic acids research **47**, D427 (2019).

[S7] S. C. Potter, A. Luciani, S. R. Eddy, Y. Park, R. Lopez, and R. D. Finn, Hmmer web server: 2018 update, Nucleic acids research **46**, W200 (2018).

[S8] K. J. Lauersen, O. Kruse, and J. H. Mussgnug, Targeted expression of nuclear transgenes in *Chlamydomonas reinhardtii* with a versatile, modular vector toolkit, Applied Microbiology and Biotechnology **99**, 3491 (2015).

[S9] C. Stringer, T. Wang, M. Michaelos, and M. Pachitariu, Cellpose: a generalist algorithm for cellular segmentation, Nature Methods **18**, 100 (2021).

[S10] C. Stringer and M. Pachitariu, Cellpose3: one-click image restoration for improved cellular segmentation, bioRxiv (2024), preprint, https://doi.org/10.1101/2024.02.10.579780.

[S11] P. Milanfar, G. C. Verghese, W. C. Karl, and A. S. Willsky, Reconstructing polygons from moments with connections to array processing, IEEE Transactions on Signal Processing **43**, 432 (1995).

[S12] G. Strang, *Introduction to Linear Algebra, Sixth Edition* (Wellesley-Cambridge Press, Philadelphia, PA, 2022).

[S13] N. Fusco, F. Maggi, and A. Pratelli, The sharp quantitative isoperimetric inequality, Annals of Mathematics , 941 (2008).

[S14] G. Polya and G. Szegö, *Isoperimetric Inequalities in Mathematical Physics* (Princeton University Press, Princeton, 1951).

[S15] L. Fejes Toth, Sur la représentation d'une population infinie par un nombre fini d'éléments, Acta Mathematica Academiae Scientiarum Hungarica **10**, 299 (1959).

[S16] D. Newman, The hexagon theorem, IEEE Transactions on Information Theory **28**, 137 (1982).

[S17] L. Atia, D. Bi, Y. Sharma, J. A. Mitchel, B. Gweon, S. A. Koehler, S. J. DeCamp, B. Lan, J. H. Kim, R. Hirsch, *et al.*, Geometric constraints during epithelial jamming, Nature Physics **14**, 613 (2018).
